# Supplementary material for: STF: Shallow-Level Temporal Feedback to Enhance Spiking Transformers
Source: arXiv:2508.00387 source file (2025-08-09)
Supplement: Supplementary file 1 [file aaai26_appendix.pdf]

| Dataset | Methods | Time Step | Clean | FGSM Maximum Perturbation | | | | PGD Iterations | | | |
|---|---|---|---|---|---|---|---|---|---|---|---|
| | | | | 0.05 | 0.1 | 0.2 | 0.3 | 5 | 10 | 30 | 50 |
| CIFAR-10 | Spikformer | 2 | 93.20 | 46.24 | 40.33 | 29.44 | 23.00 | 31.44 | 25.73 | 23.30 | 22.38 |
| | Spikformer w/ STF | 2 | **94.95 (+1.75)** | **46.69 (+0.45)** | **42.64 (+2.31)** | **34.23 (+4.79)** | **26.22 (+3.22)** | **33.72 (+2.28)** | **29.32 (+3.59)** | **27.14 (+3.84)** | **26.96 (+4.58)** |
| | Spikformer | 4 | 95.19 | 54.92 | 51.72 | 41.20 | 30.98 | 27.56 | 21.08 | 18.33 | 17.68 |
| | Spikformer w/ STF | 4 | **95.61 (+0.42)** | **58.37 (+3.45)** | **55.75 (+4.03)** | **45.40 (+4.2)** | **35.89 (+4.91)** | **30.95 (+3.39)** | **23.81 (+2.73)** | **20.54 (+2.21)** | **20.05 (+2.37)** |
| | Spikformer | 6 | 95.14 | 56.13 | 50.48 | 35.31 | 24.93 | 28.15 | 22.50 | 19.88 | 19.11 |
| | Spikformer w/ STF | 6 | **95.85 (+0.71)** | **61.33 (+5.2)** | **59.72 (+9.24)** | **50.70 (+15.39)** | **40.56 (+15.63)** | **31.37 (+3.22)** | **25.37 (+2.87)** | **22.47 (+2.59)** | **21.97 (+2.86)** |
| | Spikformer | 8 | 95.24 | 53.13 | 47.21 | 35.53 | 26.24 | 28.61 | 24.53 | 22.29 | 22.04 |
| | Spikformer w/ STF | 8 | **95.99 (+0.75)** | **60.59 (+7.46)** | **58.88 (+11.67)** | **50.19 (+14.66)** | **39.58 (+13.34)** | **32.81 (+4.20)** | **26.49 (+1.96)** | **23.44 (+1.15)** | **22.56 (+0.52)** |
| CIFAR-100 | Spikformer | 2 | 75.17 | 21.96 | 15.82 | 9.79 | 6.91 | 14.03 | 10.32 | 9.01 | 9.06 |
| | Spikformer w/ STF | 2 | **76.94 (+1.77)** | **22.10 (+0.14)** | **16.11 (+0.29)** | **10.10 (+0.31)** | **7.07 (+0.16)** | **14.06 (+0.03)** | **10.51 (+0.19)** | **9.11 (+0.10)** | **9.34 (+0.28)** |
| | Spikformer | 4 | 77.86 | 26.05 | 21.86 | 15.19 | 10.58 | 15.03 | 11.52 | 9.79 | 9.58 |
| | Spikformer w/ STF | 4 | **78.00 (+0.14)** | **26.41 (+0.36)** | **22.00 (+0.14)** | **15.75 (+0.56)** | **11.73 (+1.15)** | **15.12 (+0.09)** | **12.36 (+0.84)** | **10.48 (+0.69)** | **10.50 (+0.92)** |
| | Spikformer | 6 | 78.17 | 29.94 | 25.49 | 16.96 | 11.86 | 15.39 | 12.32 | 10.55 | **10.11** |
| | Spikformer w/ STF | 6 | **78.87 (+0.70)** | **30.68 (+0.74)** | **27.18 (+1.69)** | **20.15 (+3.19)** | **14.59 (+2.73)** | **15.93 (+0.54)** | **12.37 (+0.05)** | **10.64 (+0.09)** | 10.03 (-0.08) |
| | Spikformer | 8 | 78.22 | 31.18 | 26.34 | 18.22 | 12.77 | 15.74 | 12.55 | 10.97 | 10.67 |
| | Spikformer w/ STF | 8 | **79.14 (+0.92)** | **31.47 (+0.29)** | **28.14 (+1.80)** | **21.17 (+2.95)** | **15.90 (+3.13)** | **17.22 (+1.48)** | **13.54 (+0.99)** | **11.79 (+0.82)** | **11.58 (+0.91)** |

Table 7: Adversarial robustness comparison between Spikformer with and without STF on the CIFAR datasets.

| Dataset | Methods | Time Step | Clean | FGSM Maximum Perturbation | | | | PGD Iterations | | | |
|---|---|---|---|---|---|---|---|---|---|---|---|
| | | | | 0.05 | 0.1 | 0.2 | 0.3 | 5 | 10 | 30 | 50 |
| CIFAR-10 | SDT | 2 | 95.01 | 52.65 | 42.74 | 33.97 | 28.23 | 35.77 | 27.6 | 23.17 | 23.99 |
| | SDT w/ STF | 2 | **95.24 (+0.23)** | **52.89 (+0.24)** | **43.29 (+0.55)** | **34.22 (+0.25)** | **28.95 (+0.72)** | **36.12 (+0.35)** | **28.32 (+0.72)** | **24.74 (+1.57)** | **24.92 (+0.93)** |
| | SDT | 4 | 95.60 | 62.11 | 56.18 | 50.54 | 46.46 | 38.59 | 30.81 | 26.1 | **25.62** |
| | SDT w/ STF | 4 | **95.86 (+0.26)** | **63.91 (+1.80)** | **59.57 (+3.39)** | **53.78 (+3.24)** | **50.00 (+3.54)** | **39.01 (+0.42)** | **30.85 (+0.04)** | **26.48 (+0.38)** | 25.53 (-0.09) |
| | SDT | 6 | 96.11 | 69.31 | 66.37 | 61.13 | 57.01 | 42.29 | 34.81 | 30.45 | 28.77 |
| | SDT w/ STF | 6 | **96.23 (+0.12)** | **70.22 (+0.91)** | **67.74 (+1.37)** | **63.51 (+2.38)** | **59.74 (+2.73)** | **43.03 (+0.74)** | **35.1 (+0.29)** | **30.57 (+0.12)** | **29.6 (+0.83)** |
| | SDT | 8 | 96.24 | 70.26 | 67.94 | 63.04 | 58.28 | 42.85 | 35.42 | 30.63 | 30.16 |
| | SDT w/ STF | 8 | **96.41 (+0.17)** | **72.65 (+2.39)** | **69.06 (+1.12)** | **63.89 (+0.85)** | **59.22 (+0.94)** | **43.99 (+1.14)** | **36.37 (+0.95)** | **31.59 (+0.96)** | **30.70 (+0.54)** |
| CIFAR-100 | SDT | 2 | 77.47 | 32.29 | 26.66 | 21.63 | 18.30 | 20.73 | 15.88 | 14.82 | 14.4 |
| | SDT w/ STF | 2 | **78.21 (+0.74)** | **33.23 (+0.94)** | **27.86 (+1.20)** | **22.91 (+1.28)** | **20.02 (+1.72)** | **21.02 (+0.29)** | **16.81 (+0.93)** | **15.17 (+0.35)** | **14.83 (+0.43)** |
| | SDT | 4 | 78.40 | 37.23 | **32.97** | 27.69 | 25.02 | 23.16 | 17.91 | 16.84 | 16.25 |
| | SDT w/ STF | 4 | **79.44 (+1.04)** | **37.46 (+0.23)** | 32.60 (-0.37) | **28.52 (+0.83)** | **25.08 (+0.06)** | **23.43 (+0.27)** | **18.76 (+0.85)** | **17.30 (+0.46)** | **16.48 (+0.23)** |
| | SDT | 6 | 79.43 | 38.01 | 34.75 | 30.13 | 26.88 | 22.15 | 17.71 | 15.64 | 15.49 |
| | SDT w/ STF | 6 | **80.34 (+0.91)** | **39.39 (+1.38)** | **35.53 (+0.78)** | **31.67 (+1.54)** | **28.24 (+1.36)** | **22.80 (+0.65)** | **18.18 (+0.47)** | **16.35 (+0.71)** | **16.10 (+0.61)** |
| | SDT | 8 | 79.87 | 40.22 | 36.49 | 31.79 | 28.49 | 22.31 | 18.07 | 14.81 | 14.71 |
| | SDT w/ STF | 8 | **80.61 (+0.74)** | **40.33 (+0.11)** | **36.53 (+0.04)** | **32.42 (+0.63)** | **29.38 (+0.89)** | **22.54 (+0.23)** | **18.41 (+0.34)** | **15.90 (+1.09)** | **15.57 (+0.86)** |

Table 8: Adversarial robustness comparison between SDT with and without STF on the CIFAR datasets.

| Dataset | Methods | Time Step | Clean | FGSM Maximum Perturbation | | | | PGD Iterations | | | |
|---|---|---|---|---|---|---|---|---|---|---|---|
| | | | | 0.05 | 0.1 | 0.2 | 0.3 | 5 | 10 | 30 | 50 |
| CIFAR-10 | QKFormer | 2 | 95.79 | 59.08 | 51.57 | 43.19 | 37.19 | 31.37 | 22.11 | 16.50 | 15.45 |
| | QKFormer w/ STF | 2 | **96.02** | **59.52** | **51.85** | **43.36** | **37.31** | **31.81** | **22.23** | **17.09** | **15.86** |
| | | | **(+0.23)** | **(+0.44)** | **(+0.28)** | **(+0.17)** | **(+0.12)** | **(+0.44)** | **(+0.12)** | **(+0.59)** | **(+0.41)** |
| | QKFormer | 4 | 96.18 | 68.56 | 64.50 | 58.64 | 51.77 | 33.11 | 24.59 | 17.80 | 16.63 |
| | QKFormer w/ STF | 4 | **96.33** | **71.15** | **67.61** | **61.16** | **54.26** | **38.33** | **28.21** | **21.07** | **19.31** |
| | | | **(+0.15)** | **(+2.59)** | **(+3.11)** | **(+2.52)** | **(+2.49)** | **(+5.22)** | **(+3.62)** | **(+3.27)** | **(+2.68)** |
| | QKFormer | 6 | 96.37 | 66.07 | 61.30 | 53.19 | 45.80 | 34.21 | 24.71 | 18.28 | 17.09 |
| | QKFormer w/ STF | 6 | **96.51** | **66.88** | **64.06** | **58.61** | **52.83** | **34.43** | **25.08** | **18.47** | **17.13** |
| | | | **(+0.14)** | **(+0.81)** | **(+2.76)** | **(+5.42)** | **(+7.03)** | **(+0.22)** | **(+0.37)** | **(+0.19)** | **(+0.04)** |
| | QKFormer | 8 | 96.35 | 68.51 | 65.68 | 60.12 | 54.37 | 35.43 | 26.20 | 20.30 | **18.93** |
| | QKFormer w/ STF | 8 | **96.61** | **68.79** | **66.97** | **61.61** | **54.69** | **36.59** | **27.49** | **20.32** | 18.86 |
| | | | **(+0.26)** | **(+0.28)** | **(+1.29)** | **(+1.49)** | **(+0.32)** | **(+1.16)** | **(+1.29)** | **(+0.02)** | (-0.07) |
| CIFAR-100 | QKFormer | 2 | 79.79 | 32.63 | 28.05 | 22.98 | 18.95 | 17.25 | 12.52 | 10.15 | 9.86 |
| | QKFormer w/ STF | 2 | **80.07** | **36.21** | **31.44** | **25.42** | **21.04** | **20.44** | **15.29** | **12.62** | **12.09** |
| | | | **(+0.28)** | **(+3.58)** | **(+3.39)** | **(+2.44)** | **(+2.09)** | **(+3.19)** | **(+2.77)** | **(+2.47)** | **(+2.23)** |
| | QKFormer | 4 | 81.15 | 35.56 | 31.37 | 25.67 | 21.63 | 18.19 | 13.61 | 9.89 | 10.04 |
| | QKFormer w/ STF | 4 | **81.26** | **37.19** | **32.94** | **27.27** | **23.04** | **19.32** | **14.45** | **11.26** | **10.75** |
| | | | **(+0.11)** | **(+1.63)** | **(+1.57)** | **(+1.60)** | **(+1.41)** | **(+1.13)** | **(+0.84)** | **(+1.37)** | **(+0.71)** |
| | QKFormer | 6 | 81.35 | 36.90 | 33.39 | 28.43 | 23.97 | 18.40 | 13.32 | 9.89 | 9.10 |
| | QKFormer w/ STF | 6 | **81.51** | **38.33** | **35.27** | **30.01** | **25.42** | **20.49** | **15.41** | **11.84** | **11.13** |
| | | | **(+0.16)** | **(+1.43)** | **(+1.88)** | **(+1.58)** | **(+1.45)** | **(+2.09)** | **(+2.09)** | **(+1.95)** | **(+2.03)** |
| | QKFormer | 8 | 81.64 | 37.97 | 34.69 | 28.44 | 23.70 | 35.44 | 26.20 | 20.29 | **18.93** |
| | QKFormer w/ STF | 8 | **81.89** | **39.96** | **36.84** | **30.52** | **25.95** | **36.59** | **27.50** | **20.30** | 18.91 |
| | | | **(+0.25)** | **(+1.99)** | **(+2.15)** | **(+2.08)** | **(+2.25)** | **(+1.15)** | **(+1.30)** | **(+0.01)** | (-0.02) |

Table 9: Adversarial robustness comparison between QKFormer with and without STF on the CIFAR datasets.

| Spike Pattern | Count | Ratio |
|---|---|---|
| $[0, 0]$ | 386,181,630 | 0.78569 |
| $[0, 1]$ | 54,595,182 | 0.11107 |
| $[1, 0]$ | 0 | 0 |
| $[1, 1]$ | 50,743,188 | 0.10324 |
| Spike Entropy | 0.9637 | |
| Firing Rate | 0.1588 | |

(a) Direct Coding

| Spike Pattern | Count | Ratio |
|---|---|---|
| $[0, 0]$ | 385,766,667 | 0.78484 |
| $[0, 1]$ | 54,736,027 | 0.11136 |
| $[1, 0]$ | 0 | 0 |
| $[1, 1]$ | 51,017,306 | 0.10379 |
| Spike Entropy | 0.9662 | |
| Firing Rate | 0.1595 | |

(b) GAC Coding

| Spike Pattern | Count | Ratio |
|---|---|---|
| $[0, 0]$ | 332,652,925 | 0.67678 |
| $[0, 1]$ | 44,688,373 | 0.09092 |
| $[1, 0]$ | 42,131,763 | 0.08572 |
| $[1, 1]$ | 72,046,939 | 0.14658 |
| Spike Entropy | 1.4056 | |
| Firing Rate | 0.2349 | |

(c) IMP Coding

| Spike Pattern | Count | Ratio |
|---|---|---|
| $[0, 0]$ | 318,063,858 | 0.64710 |
| $[0, 1]$ | 70,499,779 | 0.14343 |
| $[1, 0]$ | 29,936,350 | 0.06091 |
| $[1, 1]$ | 73,020,013 | 0.14856 |
| Spike Entropy | 1.4627 | |
| Firing Rate | 0.2507 | |

(d) STF (Ours)

Table 10: Distribution of the spike patterns in the encoding layer of Spikformer with different schemes on CIFAR-10 at $T = 2$.

| Spike Pattern | Count | Ratio |
|---|---|---|
| $[0,0,0,0]$ | 342,242,368 | 0.69629 |
| $[0,0,0,1]$ | 13,510,753 | 0.02749 |
| $[0,0,1,0]$ | 28,708,328 | 0.05841 |
| $[0,0,1,1]$ | 0 | 0 |
| $[0,1,0,0]$ | 0 | 0 |
| $[0,1,0,1]$ | 56,695,620 | 0.11535 |
| $[0,1,1,0]$ | 0 | 0 |
| $[0,1,1,1]$ | 0 | 0 |
| $[1,0,0,0]$ | 0 | 0 |
| $[1,0,0,1]$ | 0 | 0 |
| $[1,0,1,0]$ | 0 | 0 |
| $[1,0,1,1]$ | 0 | 0 |
| $[1,1,0,0]$ | 0 | 0 |
| $[1,1,0,1]$ | 0 | 0 |
| $[1,1,1,0]$ | 0 | 0 |
| $[1,1,1,1]$ | 50,362,931 | 0.10246 |
| Spike Entropy | 1.4417 | |
| Firing Rate | 0.1816 | |

(a) Direct Coding

| Spike Pattern | Count | Ratio |
|---|---|---|
| $[0,0,0,0]$ | 349,113,731 | 0.71027 |
| $[0,0,0,1]$ | 12,453,653 | 0.02534 |
| $[0,0,1,0]$ | 26,487,893 | 0.05389 |
| $[0,0,1,1]$ | 0 | 0 |
| $[0,1,0,0]$ | 0 | 0 |
| $[0,1,0,1]$ | 53,701,975 | 0.10926 |
| $[0,1,1,0]$ | 0 | 0 |
| $[0,1,1,1]$ | 0 | 0 |
| $[1,0,0,0]$ | 0 | 0 |
| $[1,0,0,1]$ | 0 | 0 |
| $[1,0,1,0]$ | 0 | 0 |
| $[1,0,1,1]$ | 0 | 0 |
| $[1,1,0,0]$ | 0 | 0 |
| $[1,1,0,1]$ | 0 | 0 |
| $[1,1,1,0]$ | 0 | 0 |
| $[1,1,1,1]$ | 49,762,748 | 0.10124 |
| Spike Entropy | 1.3955 | |
| Firing Rate | 0.1757 | |

(b) GAC Coding

| Spike Pattern | Count | Ratio |
|---|---|---|
| $[0,0,0,0]$ | 331,272,166 | 0.67397 |
| $[0,0,0,1]$ | 7,127,049 | 0.01450 |
| $[0,0,1,0]$ | 16,387,942 | 0.03334 |
| $[0,0,1,1]$ | 0 | 0 |
| $[0,1,0,0]$ | 24,011,229 | 0.04885 |
| $[0,1,0,1]$ | 18,759,892 | 0.03817 |
| $[0,1,1,0]$ | 0 | 0 |
| $[0,1,1,1]$ | 0 | 0 |
| $[1,0,0,0]$ | 0 | 0 |
| $[1,0,0,1]$ | 0 | 0 |
| $[1,0,1,0]$ | 37,373,113 | 0.07604 |
| $[1,0,1,1]$ | 0 | 0 |
| $[1,1,0,0]$ | 0 | 0 |
| $[1,1,0,1]$ | 0 | 0 |
| $[1,1,1,0]$ | 0 | 0 |
| $[1,1,1,1]$ | 56,588,609 | 0.11513 |
| Spike Entropy | 1.6701 | |
| Firing Rate | 0.1964 | |

(c) IMP Coding

| Spike Pattern | Count | Ratio |
|---|---|---|
| $[0,0,0,0]$ | 265,198,402 | 0.53955 |
| $[0,0,0,1]$ | 19,567,140 | 0.03981 |
| $[0,0,1,0]$ | 33,923,411 | 0.06902 |
| $[0,0,1,1]$ | 7,457,890 | 0.01517 |
| $[0,1,0,0]$ | 28,667,675 | 0.05833 |
| $[0,1,0,1]$ | 24,183,612 | 0.04920 |
| $[0,1,1,0]$ | 11,907,156 | 0.02423 |
| $[0,1,1,1]$ | 15,956,240 | 0.03246 |
| $[1,0,0,0]$ | 8,005,800 | 0.01629 |
| $[1,0,0,1]$ | 2,780,431 | 0.00566 |
| $[1,0,1,0]$ | 7,693,307 | 0.01565 |
| $[1,0,1,1]$ | 3,815,101 | 0.00776 |
| $[1,1,0,0]$ | 3,338,439 | 0.00679 |
| $[1,1,0,1]$ | 5,733,335 | 0.01166 |
| $[1,1,1,0]$ | 4,863,576 | 0.00989 |
| $[1,1,1,1]$ | 48,428,485 | 0.09853 |
| Spike Entropy | 2.5732 | |
| Firing Rate | 0.2491 | |

(d) STF (Ours)

Table 11: Distribution of the spike patterns in the encoding layer of Spikformer with different schemes on CIFAR-10 at $T = 4$.

| Spike Pattern | Count | Ratio | Spike Pattern | Count | Ratio |
|---|---|---|---|---|---|
| $[0, 0, 0, 0, 0, 0]$ | 342,373,731 | 0.69656 | $[1, 0, 0, 0, 0, 0]$ | 0 | 0 |
| $[0, 0, 0, 0, 0, 1]$ | 3,111,285 | 0.00633 | $[1, 0, 0, 0, 0, 1]$ | 0 | 0 |
| $[0, 0, 0, 0, 1, 0]$ | 6,282,613 | 0.01278 | $[1, 0, 0, 0, 1, 0]$ | 0 | 0 |
| $[0, 0, 0, 1, 0, 0]$ | 13,225,515 | 0.02691 | $[1, 0, 0, 1, 0, 0]$ | 0 | 0 |
| $[0, 0, 0, 1, 0, 1]$ | 0 | 0 | $[1, 0, 0, 1, 0, 1]$ | 0 | 0 |
| $[0, 0, 0, 0, 0, 1, 1]$ | 0 | 0 | $[1, 0, 0, 0, 1, 1]$ | 0 | 0 |
| $[0, 0, 1, 1, 0]$ | 0 | 0 | $[1, 0, 0, 1, 1, 0]$ | 0 | 0 |
| $[0, 0, 0, 1, 1, 1]$ | 0 | 0 | $[1, 0, 0, 1, 1, 1]$ | 0 | 0 |
| $[0, 0, 1, 0, 0, 0]$ | 0 | 0 | $[1, 0, 1, 0, 0, 0]$ | 0 | 0 |
| $[0, 0, 1, 0, 0, 1]$ | 27,506,090 | 0.05596 | $[1, 0, 1, 0, 0, 1]$ | 0 | 0 |
| $[0, 0, 1, 0, 1, 0]$ | 0 | 0 | $[1, 0, 1, 0, 1, 0]$ | 0 | 0 |
| $[0, 0, 1, 0, 1, 1]$ | 0 | 0 | $[1, 0, 1, 0, 1, 1]$ | 0 | 0 |
| $[0, 0, 1, 1, 0, 0]$ | 0 | 0 | $[1, 0, 1, 1, 0, 0]$ | 0 | 0 |
| $[0, 0, 1, 1, 0, 1]$ | 0 | 0 | $[1, 0, 1, 1, 0, 1]$ | 0 | 0 |
| $[0, 0, 1, 1, 1, 0]$ | 0 | 0 | $[1, 0, 1, 1, 1, 0]$ | 0 | 0 |
| $[0, 0, 1, 1, 1, 1]$ | 0 | 0 | $[1, 0, 1, 1, 1, 1]$ | 0 | 0 |
| $[0, 1, 0, 0, 0, 0]$ | 0 | 0 | $[1, 1, 0, 0, 0, 0]$ | 0 | 0 |
| $[0, 1, 0, 0, 0, 1]$ | 0 | 0 | $[1, 1, 0, 0, 0, 1]$ | 0 | 0 |
| $[0, 1, 0, 0, 1, 0]$ | 0 | 0 | $[1, 1, 0, 0, 1, 0]$ | 0 | 0 |
| $[0, 1, 0, 0, 1, 1]$ | 0 | 0 | $[1, 1, 0, 0, 1, 1]$ | 0 | 0 |
| $[0, 1, 0, 1, 0, 0]$ | 0 | 0 | $[1, 1, 0, 1, 0, 0]$ | 0 | 0 |
| $[0, 1, 0, 1, 0, 1]$ | 52,721,780 | 0.10726 | $[1, 1, 0, 1, 0, 1]$ | 0 | 0 |
| $[0, 1, 0, 1, 1, 0]$ | 0 | 0 | $[1, 1, 0, 1, 1, 0]$ | 0 | 0 |
| $[0, 1, 0, 1, 1, 1]$ | 0 | 0 | $[1, 1, 0, 1, 1, 1]$ | 0 | 0 |
| $[0, 1, 1, 0, 0, 0]$ | 0 | 0 | $[1, 1, 1, 0, 0, 0]$ | 0 | 0 |
| $[0, 1, 1, 0, 0, 1]$ | 0 | 0 | $[1, 1, 1, 0, 0, 1]$ | 0 | 0 |
| $[0, 1, 1, 0, 1, 0]$ | 0 | 0 | $[1, 1, 1, 0, 1, 0]$ | 0 | 0 |
| $[0, 1, 1, 0, 1, 1]$ | 0 | 0 | $[1, 1, 1, 0, 1, 1]$ | 0 | 0 |
| $[0, 1, 1, 1, 0, 0]$ | 0 | 0 | $[1, 1, 1, 1, 0, 0]$ | 0 | 0 |
| $[0, 1, 1, 1, 0, 1]$ | 0 | 0 | $[1, 1, 1, 1, 0, 1]$ | 0 | 0 |
| $[0, 1, 1, 1, 1, 0]$ | 0 | 0 | $[1, 1, 1, 1, 1, 0]$ | 0 | 0 |
| $[0, 1, 1, 1, 1, 1]$ | 0 | 0 | $[1, 1, 1, 1, 1, 1]$ | 46,298,986 | 0.0942 |
| Spike Entropy | | | 1.5296 | | |
| Firing Rate | | | 0.1742 | | |

Table 12: Distribution of the spike patterns in the encoding layer of Spikformer with direct coding on CIFAR-10 at $T = 6$.

| Spike Pattern | Count | Ratio | Spike Pattern | Count | Ratio |
|---|---|---|---|---|---|
| $[0,0,0,0,0,0]$ | 343,464,329 | 0.69878 | $[1,0,0,0,0,0]$ | 0 | 0 |
| $[0,0,0,0,0,1]$ | 2,946,366 | 0.00599 | $[1,0,0,0,0,1]$ | 0 | 0 |
| $[0,0,0,0,1,0]$ | 6,005,346 | 0.01222 | $[1,0,0,0,1,0]$ | 0 | 0 |
| $[0,0,0,0,1,1]$ | 0 | 0 | $[1,0,0,0,1,1]$ | 0 | 0 |
| $[0,0,0,1,0,0]$ | 12,401,887 | 0.02523 | $[1,0,0,1,0,0]$ | 0 | 0 |
| $[0,0,0,1,0,1]$ | 0 | 0 | $[1,0,0,1,0,1]$ | 0 | 0 |
| $[0,0,0,1,1,0]$ | 0 | 0 | $[1,0,0,1,1,0]$ | 0 | 0 |
| $[0,0,0,1,1,1]$ | 0 | 0 | $[1,0,0,1,1,1]$ | 0 | 0 |
| $[0,0,1,0,0,0]$ | 0 | 0 | $[1,0,1,0,0,0]$ | 0 | 0 |
| $[0,0,1,0,0,1]$ | 26,284,530 | 0.05348 | $[1,0,1,0,0,1]$ | 0 | 0 |
| $[0,0,1,0,1,0]$ | 0 | 0 | $[1,0,1,0,1,0]$ | 0 | 0 |
| $[0,0,1,0,1,1]$ | 0 | 0 | $[1,0,1,0,1,1]$ | 0 | 0 |
| $[0,0,1,1,0,0]$ | 0 | 0 | $[1,0,1,1,0,0]$ | 0 | 0 |
| $[0,0,1,1,0,1]$ | 0 | 0 | $[1,0,1,1,0,1]$ | 0 | 0 |
| $[0,0,1,1,1,0]$ | 0 | 0 | $[1,0,1,1,1,0]$ | 0 | 0 |
| $[0,0,1,1,1,1]$ | 0 | 0 | $[1,0,1,1,1,1]$ | 0 | 0 |
| $[0,1,0,0,0,0]$ | 0 | 0 | $[1,1,0,0,0,0]$ | 0 | 0 |
| $[0,1,0,0,0,1]$ | 0 | 0 | $[1,1,0,0,0,1]$ | 0 | 0 |
| $[0,1,0,0,1,0]$ | 0 | 0 | $[1,1,0,0,1,0]$ | 0 | 0 |
| $[0,1,0,0,1,1]$ | 0 | 0 | $[1,1,0,0,1,1]$ | 0 | 0 |
| $[0,1,0,1,0,0]$ | 0 | 0 | $[1,1,0,1,0,0]$ | 0 | 0 |
| $[0,1,0,1,0,1]$ | 53,059,139 | 0.10795 | $[1,1,0,1,0,1]$ | 0 | 0 |
| $[0,1,0,1,1,0]$ | 0 | 0 | $[1,1,0,1,1,0]$ | 0 | 0 |
| $[0,1,0,1,1,1]$ | 0 | 0 | $[1,1,0,1,1,1]$ | 0 | 0 |
| $[0,1,1,0,0,0]$ | 0 | 0 | $[1,1,1,0,0,0]$ | 0 | 0 |
| $[0,1,1,0,0,1]$ | 0 | 0 | $[1,1,1,0,0,1]$ | 0 | 0 |
| $[0,1,1,0,1,0]$ | 0 | 0 | $[1,1,1,0,1,0]$ | 0 | 0 |
| $[0,1,1,0,1,1]$ | 0 | 0 | $[1,1,1,0,1,1]$ | 0 | 0 |
| $[0,1,1,1,0,0]$ | 0 | 0 | $[1,1,1,1,0,0]$ | 0 | 0 |
| $[0,1,1,1,0,1]$ | 0 | 0 | $[1,1,1,1,0,1]$ | 0 | 0 |
| $[0,1,1,1,1,0]$ | 0 | 0 | $[1,1,1,1,1,0]$ | 0 | 0 |
| $[0,1,1,1,1,1]$ | 0 | 0 | $[1,1,1,1,1,1]$ | 47,358,403 | 0.09635 |
| Spike Entropy | | | 1.5150 | | |
| Firing Rate | | | 0.1754 | | |

Table 13: Distribution of the spike patterns in the encoding layer of Spikformer with GAC coding on CIFAR-10 at $T = 6$.

| Spike Pattern | Count | Ratio | Spike Pattern | Count | Ratio |
|---|---|---|---|---|---|
| $[0, 0, 0, 0, 0, 0]$ | 338,159,121 | 0.68799 | $[1, 0, 0, 0, 0, 0]$ | 0 | 0 |
| $[0, 0, 0, 0, 0, 1]$ | 1,639,282 | 0.00333 | $[1, 0, 0, 0, 0, 1]$ | 0 | 0 |
| $[0, 0, 0, 0, 1, 0]$ | 3,392,152 | 0.00690 | $[1, 0, 0, 0, 1, 0]$ | 0 | 0 |
| $[0, 0, 0, 0, 1, 1]$ | 0 | 0 | $[1, 0, 0, 0, 1, 1]$ | 0 | 0 |
| $[0, 0, 0, 1, 0, 0]$ | 7,176,057 | 0.01460 | $[1, 0, 0, 1, 0, 0]$ | 0 | 0 |
| $[0, 0, 0, 1, 0, 1]$ | 0 | 0 | $[1, 0, 0, 1, 0, 1]$ | 0 | 0 |
| $[0, 0, 0, 1, 1, 0]$ | 0 | 0 | $[1, 0, 0, 1, 1, 0]$ | 0 | 0 |
| $[0, 0, 0, 1, 1, 1]$ | 0 | 0 | $[1, 0, 0, 1, 1, 1]$ | 0 | 0 |
| $[0, 0, 1, 0, 0, 0]$ | 12,294,224 | 0.02501 | $[1, 0, 1, 0, 0, 0]$ | 0 | 0 |
| $[0, 0, 1, 0, 0, 1]$ | 4,026,400 | 0.00819 | $[1, 0, 1, 0, 0, 1]$ | 0 | 0 |
| $[0, 0, 1, 0, 1, 0]$ | 0 | 0 | $[1, 0, 1, 0, 1, 0]$ | 34,806,496 | 0.07081 |
| $[0, 0, 1, 0, 1, 1]$ | 0 | 0 | $[1, 0, 1, 0, 1, 1]$ | 0 | 0 |
| $[0, 0, 1, 1, 0, 0]$ | 0 | 0 | $[1, 0, 1, 1, 0, 0]$ | 0 | 0 |
| $[0, 0, 1, 1, 0, 1]$ | 0 | 0 | $[1, 0, 1, 1, 0, 1]$ | 0 | 0 |
| $[0, 0, 1, 1, 1, 0]$ | 0 | 0 | $[1, 0, 1, 1, 1, 0]$ | 0 | 0 |
| $[0, 0, 1, 1, 1, 1]$ | 0 | 0 | $[1, 0, 1, 1, 1, 1]$ | 0 | 0 |
| $[0, 1, 0, 0, 0, 0]$ | 0 | 0 | $[1, 1, 0, 0, 0, 0]$ | 0 | 0 |
| $[0, 1, 0, 0, 0, 1]$ | 105,634 | 0.00021 | $[1, 1, 0, 0, 0, 1]$ | 0 | 0 |
| $[0, 1, 0, 0, 1, 0]$ | 23,232,901 | 0.04727 | $[1, 1, 0, 0, 1, 0]$ | 0 | 0 |
| $[0, 1, 0, 0, 1, 1]$ | 0 | 0 | $[1, 1, 0, 0, 1, 1]$ | 0 | 0 |
| $[0, 1, 0, 1, 0, 0]$ | 0 | 0 | $[1, 1, 0, 1, 0, 0]$ | 0 | 0 |
| $[0, 1, 0, 1, 0, 1]$ | 17,930,876 | 0.03648 | $[1, 1, 0, 1, 0, 1]$ | 0 | 0 |
| $[0, 1, 0, 1, 1, 0]$ | 0 | 0 | $[1, 1, 0, 1, 1, 0]$ | 0 | 0 |
| $[0, 1, 0, 1, 1, 1]$ | 0 | 0 | $[1, 1, 0, 1, 1, 1]$ | 0 | 0 |
| $[0, 1, 1, 0, 0, 0]$ | 0 | 0 | $[1, 1, 1, 0, 0, 0]$ | 0 | 0 |
| $[0, 1, 1, 0, 0, 1]$ | 0 | 0 | $[1, 1, 1, 0, 0, 1]$ | 0 | 0 |
| $[0, 1, 1, 0, 1, 0]$ | 0 | 0 | $[1, 1, 1, 0, 1, 0]$ | 0 | 0 |
| $[0, 1, 1, 0, 1, 1]$ | 0 | 0 | $[1, 1, 1, 0, 1, 1]$ | 0 | 0 |
| $[0, 1, 1, 1, 0, 0]$ | 0 | 0 | $[1, 1, 1, 1, 0, 0]$ | 0 | 0 |
| $[0, 1, 1, 1, 0, 1]$ | 0 | 0 | $[1, 1, 1, 1, 0, 1]$ | 0 | 0 |
| $[0, 1, 1, 1, 1, 0]$ | 0 | 0 | $[1, 1, 1, 1, 1, 0]$ | 0 | 0 |
| $[0, 1, 1, 1, 1, 1]$ | 0 | 0 | $[1, 1, 1, 1, 1, 1]$ | 48,756,857 | 0.09920 |
| Spike Entropy | | | 1.7133 | | |
| Firing Rate | | | 0.1797 | | |

Table 14: Distribution of the spike patterns in the encoding layer of Spikformer with IMP coding on CIFAR-10 at $T = 6$.

| Spike Pattern | Count | Ratio | Spike Pattern | Count | Ratio |
|---|---|---|---|---|---|
| $[0,0,0,0,0,0]$ | 153,390,794 | 0.31207 | $[1,0,0,0,0,0]$ | 13,437,249 | 0.02734 |
| $[0,0,0,0,0,1]$ | 17,672,955 | 0.03596 | $[1,0,0,0,0,1]$ | 1,539,807 | 0.00313 |
| $[0,0,0,0,1,0]$ | 21,481,933 | 0.04371 | $[1,0,0,0,1,0]$ | 1,668,172 | 0.00339 |
| $[0,0,0,0,1,1]$ | 4,090,165 | 0.00832 | $[1,0,0,0,1,1]$ | 367,067 | 0.00075 |
| $[0,0,0,1,0,0]$ | 25,066,475 | 0.05100 | $[1,0,0,1,0,0]$ | 21,684,054 | 0.04412 |
| $[0,0,0,1,0,1]$ | 4,208,713 | 0.00856 | $[1,0,0,1,0,1]$ | 3,148,724 | 0.00641 |
| $[0,0,0,1,1,0]$ | 5,314,403 | 0.01081 | $[1,0,0,1,1,0]$ | 3,829,962 | 0.00779 |
| $[0,0,0,1,1,1]$ | 1,395,765 | 0.00284 | $[1,0,0,1,1,1]$ | 879,695 | 0.00179 |
| $[0,0,1,0,0,0]$ | 24,662,353 | 0.05018 | $[1,0,1,0,0,0]$ | 2,519,839 | 0.00513 |
| $[0,0,1,0,0,1]$ | 28,702,361 | 0.05840 | $[1,0,1,0,0,1]$ | 2,557,085 | 0.00520 |
| $[0,0,1,0,1,0]$ | 3,846,168 | 0.00783 | $[1,0,1,0,1,0]$ | 388,368 | 0.00079 |
| $[0,0,1,0,1,1]$ | 5,584,658 | 0.01136 | $[1,0,1,0,1,1]$ | 502,201 | 0.00102 |
| $[0,0,1,1,0,0]$ | 4,763,066 | 0.00969 | $[1,0,1,1,0,0]$ | 4,483,259 | 0.00912 |
| $[0,0,1,1,0,1]$ | 6,549,139 | 0.01332 | $[1,0,1,1,0,1]$ | 7,232,276 | 0.01471 |
| $[0,0,1,1,1,0]$ | 1,180,092 | 0.00240 | $[1,0,1,1,1,0]$ | 919,458 | 0.00187 |
| $[0,0,1,1,1,1]$ | 1,815,570 | 0.00369 | $[1,0,1,1,1,1]$ | 1,597,980 | 0.00325 |
| $[0,1,0,0,0,0]$ | 18,269,651 | 0.03717 | $[1,1,0,0,0,0]$ | 2,522,659 | 0.00513 |
| $[0,1,0,0,0,1]$ | 2,068,725 | 0.00421 | $[1,1,0,0,0,1]$ | 314,479 | 0.00064 |
| $[0,1,0,0,1,0]$ | 24,728,089 | 0.05031 | $[1,1,0,0,1,0]$ | 2,570,239 | 0.00523 |
| $[0,1,0,0,1,1]$ | 3,734,288 | 0.00760 | $[1,1,0,0,1,1]$ | 443,169 | 0.00090 |
| $[0,1,0,1,0,0]$ | 3,142,395 | 0.00639 | $[1,1,0,1,0,0]$ | 3,455,308 | 0.00703 |
| $[0,1,0,1,0,1]$ | 560,545 | 0.00114 | $[1,1,0,1,0,1]$ | 550,655 | 0.00112 |
| $[0,1,0,1,1,0]$ | 5,397,830 | 0.01098 | $[1,1,0,1,1,0]$ | 6,574,824 | 0.01338 |
| $[0,1,0,1,1,1]$ | 1,139,751 | 0.00232 | $[1,1,0,1,1,1]$ | 1,149,593 | 0.00234 |
| $[0,1,1,0,0,0]$ | 4,462,547 | 0.00908 | $[1,1,1,0,0,0]$ | 589,074 | 0.00120 |
| $[0,1,1,0,0,1]$ | 4,297,173 | 0.00874 | $[1,1,1,0,0,1]$ | 565,157 | 0.00115 |
| $[0,1,1,0,1,0]$ | 5,386,879 | 0.01096 | $[1,1,1,0,1,0]$ | 624,925 | 0.00127 |
| $[0,1,1,0,1,1]$ | 8,595,064 | 0.01749 | $[1,1,1,0,1,1]$ | 884,239 | 0.00180 |
| $[0,1,1,1,0,0]$ | 972,876 | 0.00198 | $[1,1,1,1,0,0]$ | 1,000,862 | 0.00204 |
| $[0,1,1,1,0,1]$ | 1,077,323 | 0.00219 | $[1,1,1,1,0,1]$ | 1,295,744 | 0.00264 |
| $[0,1,1,1,1,0]$ | 1,391,814 | 0.00283 | $[1,1,1,1,1,0]$ | 1,625,378 | 0.00331 |
| $[0,1,1,1,1,1]$ | 2,334,636 | 0.00475 | $[1,1,1,1,1,1]$ | 3,314,303 | 0.00674 |
| Spike Entropy | | | 4.3685 | | |
| Firing Rate | | | 0.2438 | | |

Table 15: Distribution of the spike patterns in the encoding layer of Spikformer with STF on CIFAR-10 at $T = 6$.

| Spike Pattern | Count | Ratio | Spike Pattern | Count | Ratio |
|---|---|---|---|---|---|
| [0, 0, 0, 0, 0, 0, 0, 0] | 325,647,136 | 0.66253 | [1, 0, 0, 0, 0, 0, 0, 0] | 0 | 0 |
| [0, 0, 0, 0, 0, 0, 0, 1] | 780,771 | 0.00159 | [1, 0, 0, 0, 0, 0, 0, 1] | 0 | 0 |
| [0, 0, 0, 0, 0, 0, 1, 0] | 1,549,957 | 0.00315 | [1, 0, 0, 0, 0, 0, 1, 0] | 0 | 0 |
| [0, 0, 0, 0, 0, 0, 1, 1] | 0 | 0 | [1, 0, 0, 0, 0, 0, 1, 1] | 0 | 0 |
| [0, 0, 0, 0, 0, 1, 0, 0] | 3,343,140 | 0.0068 | [1, 0, 0, 0, 0, 1, 0, 0] | 0 | 0 |
| [0, 0, 0, 0, 0, 1, 0, 1] | 0 | 0 | [1, 0, 0, 0, 0, 1, 0, 1] | 0 | 0 |
| [0, 0, 0, 0, 0, 1, 1, 0] | 0 | 0 | [1, 0, 0, 0, 0, 1, 1, 0] | 0 | 0 |
| [0, 0, 0, 0, 0, 1, 1, 1] | 0 | 0 | [1, 0, 0, 0, 0, 1, 1, 1] | 0 | 0 |
| [0, 0, 0, 0, 1, 0, 0, 0] | 6,669,556 | 0.01357 | [1, 0, 0, 0, 1, 0, 0, 0] | 0 | 0 |
| [0, 0, 0, 0, 1, 0, 0, 1] | 0 | 0 | [1, 0, 0, 0, 1, 0, 0, 1] | 0 | 0 |
| [0, 0, 0, 0, 1, 0, 1, 0] | 0 | 0 | [1, 0, 0, 0, 1, 0, 1, 0] | 0 | 0 |
| [0, 0, 0, 0, 1, 0, 1, 1] | 0 | 0 | [1, 0, 0, 0, 1, 0, 1, 1] | 0 | 0 |
| [0, 0, 0, 0, 1, 1, 0, 0] | 0 | 0 | [1, 0, 0, 0, 1, 1, 0, 0] | 0 | 0 |
| [0, 0, 0, 0, 1, 1, 0, 1] | 0 | 0 | [1, 0, 0, 0, 1, 1, 0, 1] | 0 | 0 |
| [0, 0, 0, 0, 1, 1, 1, 0] | 0 | 0 | [1, 0, 0, 0, 1, 1, 1, 0] | 0 | 0 |
| [0, 0, 0, 0, 1, 1, 1, 1] | 0 | 0 | [1, 0, 0, 0, 1, 1, 1, 1] | 0 | 0 |
| [0, 0, 0, 1, 0, 0, 0, 0] | 0 | 0 | [1, 0, 0, 1, 0, 0, 0, 0] | 0 | 0 |
| [0, 0, 0, 1, 0, 0, 0, 1] | 13,888,765 | 0.02826 | [1, 0, 0, 1, 0, 0, 0, 1] | 0 | 0 |
| [0, 0, 0, 1, 0, 0, 1, 0] | 0 | 0 | [1, 0, 0, 1, 0, 0, 1, 0] | 0 | 0 |
| [0, 0, 0, 1, 0, 0, 1, 1] | 0 | 0 | [1, 0, 0, 1, 0, 0, 1, 1] | 0 | 0 |
| [0, 0, 0, 1, 0, 1, 0, 0] | 0 | 0 | [1, 0, 0, 1, 0, 1, 0, 0] | 0 | 0 |
| [0, 0, 0, 1, 0, 1, 0, 1] | 0 | 0 | [1, 0, 0, 1, 0, 1, 0, 1] | 0 | 0 |
| [0, 0, 0, 1, 0, 1, 1, 0] | 0 | 0 | [1, 0, 0, 1, 0, 1, 1, 0] | 0 | 0 |
| [0, 0, 0, 1, 0, 1, 1, 1] | 0 | 0 | [1, 0, 0, 1, 0, 1, 1, 1] | 0 | 0 |
| [0, 0, 0, 1, 1, 0, 0, 0] | 0 | 0 | [1, 0, 0, 1, 1, 0, 0, 0] | 0 | 0 |
| [0, 0, 0, 1, 1, 0, 0, 1] | 0 | 0 | [1, 0, 0, 1, 1, 0, 0, 1] | 0 | 0 |
| [0, 0, 0, 1, 1, 0, 1, 0] | 0 | 0 | [1, 0, 0, 1, 1, 0, 1, 0] | 0 | 0 |
| [0, 0, 0, 1, 1, 0, 1, 1] | 0 | 0 | [1, 0, 0, 1, 1, 0, 1, 1] | 0 | 0 |
| [0, 0, 0, 1, 1, 1, 0, 0] | 0 | 0 | [1, 0, 0, 1, 1, 1, 0, 0] | 0 | 0 |
| [0, 0, 0, 1, 1, 1, 0, 1] | 0 | 0 | [1, 0, 0, 1, 1, 1, 0, 1] | 0 | 0 |
| [0, 0, 0, 1, 1, 1, 1, 0] | 0 | 0 | [1, 0, 0, 1, 1, 1, 1, 0] | 0 | 0 |
| [0, 0, 0, 1, 1, 1, 1, 1] | 0 | 0 | [1, 0, 0, 1, 1, 1, 1, 1] | 0 | 0 |
| [0, 0, 1, 0, 0, 0, 0, 0] | 0 | 0 | [1, 0, 1, 0, 0, 0, 0, 0] | 0 | 0 |
| [0, 0, 1, 0, 0, 0, 0, 1] | 0 | 0 | [1, 0, 1, 0, 0, 0, 0, 1] | 0 | 0 |
| [0, 0, 1, 0, 0, 0, 1, 0] | 0 | 0 | [1, 0, 1, 0, 0, 0, 1, 0] | 0 | 0 |
| [0, 0, 1, 0, 0, 0, 1, 1] | 0 | 0 | [1, 0, 1, 0, 0, 0, 1, 1] | 0 | 0 |
| [0, 0, 1, 0, 0, 1, 0, 0] | 29,723,360 | 0.06047 | [1, 0, 1, 0, 0, 1, 0, 0] | 0 | 0 |
| [0, 0, 1, 0, 0, 1, 0, 1] | 0 | 0 | [1, 0, 1, 0, 0, 1, 0, 1] | 0 | 0 |
| [0, 0, 1, 0, 0, 1, 1, 0] | 0 | 0 | [1, 0, 1, 0, 0, 1, 1, 0] | 0 | 0 |
| [0, 0, 1, 0, 0, 1, 1, 1] | 0 | 0 | [1, 0, 1, 0, 0, 1, 1, 1] | 0 | 0 |
| [0, 0, 1, 0, 1, 0, 0, 0] | 0 | 0 | [1, 0, 1, 0, 1, 0, 0, 0] | 0 | 0 |
| [0, 0, 1, 0, 1, 0, 0, 1] | 0 | 0 | [1, 0, 1, 0, 1, 0, 0, 1] | 0 | 0 |
| [0, 0, 1, 0, 1, 0, 1, 0] | 0 | 0 | [1, 0, 1, 0, 1, 0, 1, 0] | 0 | 0 |
| [0, 0, 1, 0, 1, 0, 1, 1] | 0 | 0 | [1, 0, 1, 0, 1, 0, 1, 1] | 0 | 0 |
| [0, 0, 1, 0, 1, 1, 0, 0] | 0 | 0 | [1, 0, 1, 0, 1, 1, 0, 0] | 0 | 0 |
| [0, 0, 1, 0, 1, 1, 0, 1] | 0 | 0 | [1, 0, 1, 0, 1, 1, 0, 1] | 0 | 0 |
| [0, 0, 1, 0, 1, 1, 1, 0] | 0 | 0 | [1, 0, 1, 0, 1, 1, 1, 0] | 0 | 0 |
| [0, 0, 1, 0, 1, 1, 1, 1] | 0 | 0 | [1, 0, 1, 0, 1, 1, 1, 1] | 0 | 0 |
| [0, 0, 1, 1, 0, 0, 0, 0] | 0 | 0 | [1, 0, 1, 1, 0, 0, 0, 0] | 0 | 0 |
| [0, 0, 1, 1, 0, 0, 0, 1] | 0 | 0 | [1, 0, 1, 1, 0, 0, 0, 1] | 0 | 0 |
| [0, 0, 1, 1, 0, 0, 1, 0] | 0 | 0 | [1, 0, 1, 1, 0, 0, 1, 0] | 0 | 0 |
| [0, 0, 1, 1, 0, 0, 1, 1] | 0 | 0 | [1, 0, 1, 1, 0, 0, 1, 1] | 0 | 0 |
| [0, 0, 1, 1, 0, 1, 0, 0] | 0 | 0 | [1, 0, 1, 1, 0, 1, 0, 0] | 0 | 0 |
| [0, 0, 1, 1, 0, 1, 0, 1] | 0 | 0 | [1, 0, 1, 1, 0, 1, 0, 1] | 0 | 0 |

*Continued on next page*

| Spike Pattern | Count | Ratio | Spike Pattern | Count | Ratio |
|---|---|---|---|---|---|
| [0, 0, 1, 1, 0, 1, 1, 0] | 0 | 0 | [1, 0, 1, 1, 0, 1, 1, 0] | 0 | 0 |
| [0, 0, 1, 1, 0, 1, 1, 1] | 0 | 0 | [1, 0, 1, 1, 0, 1, 1, 1] | 0 | 0 |
| [0, 0, 1, 1, 1, 0, 0, 0] | 0 | 0 | [1, 0, 1, 1, 1, 0, 0, 0] | 0 | 0 |
| [0, 0, 1, 1, 1, 0, 0, 1] | 0 | 0 | [1, 0, 1, 1, 1, 0, 0, 1] | 0 | 0 |
| [0, 0, 1, 1, 1, 0, 1, 0] | 0 | 0 | [1, 0, 1, 1, 1, 0, 1, 0] | 0 | 0 |
| [0, 0, 1, 1, 1, 0, 1, 1] | 0 | 0 | [1, 0, 1, 1, 1, 0, 1, 1] | 0 | 0 |
| [0, 0, 1, 1, 1, 1, 0, 0] | 0 | 0 | [1, 0, 1, 1, 1, 1, 0, 0] | 0 | 0 |
| [0, 0, 1, 1, 1, 1, 0, 1] | 0 | 0 | [1, 0, 1, 1, 1, 1, 0, 1] | 0 | 0 |
| [0, 0, 1, 1, 1, 1, 1, 0] | 0 | 0 | [1, 0, 1, 1, 1, 1, 1, 0] | 0 | 0 |
| [0, 0, 1, 1, 1, 1, 1, 1] | 0 | 0 | [1, 0, 1, 1, 1, 1, 1, 1] | 0 | 0 |
| [0, 1, 0, 0, 0, 0, 0, 0] | 0 | 0 | [1, 1, 0, 0, 0, 0, 0, 0] | 0 | 0 |
| [0, 1, 0, 0, 0, 0, 0, 1] | 0 | 0 | [1, 1, 0, 0, 0, 0, 0, 1] | 0 | 0 |
| [0, 1, 0, 0, 0, 0, 1, 0] | 0 | 0 | [1, 1, 0, 0, 0, 0, 1, 0] | 0 | 0 |
| [0, 1, 0, 0, 0, 0, 1, 1] | 0 | 0 | [1, 1, 0, 0, 0, 0, 1, 1] | 0 | 0 |
| [0, 1, 0, 0, 0, 1, 0, 0] | 0 | 0 | [1, 1, 0, 0, 0, 1, 0, 0] | 0 | 0 |
| [0, 1, 0, 0, 0, 1, 0, 1] | 0 | 0 | [1, 1, 0, 0, 0, 1, 0, 1] | 0 | 0 |
| [0, 1, 0, 0, 0, 1, 1, 0] | 0 | 0 | [1, 1, 0, 0, 0, 1, 1, 0] | 0 | 0 |
| [0, 1, 0, 0, 0, 1, 1, 1] | 0 | 0 | [1, 1, 0, 0, 0, 1, 1, 1] | 0 | 0 |
| [0, 1, 0, 0, 1, 0, 0, 0] | 0 | 0 | [1, 1, 0, 0, 1, 0, 0, 0] | 0 | 0 |
| [0, 1, 0, 0, 1, 0, 0, 1] | 0 | 0 | [1, 1, 0, 0, 1, 0, 0, 1] | 0 | 0 |
| [0, 1, 0, 0, 1, 0, 1, 0] | 0 | 0 | [1, 1, 0, 0, 1, 0, 1, 0] | 0 | 0 |
| [0, 1, 0, 0, 1, 0, 1, 1] | 0 | 0 | [1, 1, 0, 0, 1, 0, 1, 1] | 0 | 0 |
| [0, 1, 0, 0, 1, 1, 0, 0] | 0 | 0 | [1, 1, 0, 0, 1, 1, 0, 0] | 0 | 0 |
| [0, 1, 0, 0, 1, 1, 0, 1] | 0 | 0 | [1, 1, 0, 0, 1, 1, 0, 1] | 0 | 0 |
| [0, 1, 0, 0, 1, 1, 1, 0] | 0 | 0 | [1, 1, 0, 0, 1, 1, 1, 0] | 0 | 0 |
| [0, 1, 0, 0, 1, 1, 1, 1] | 0 | 0 | [1, 1, 0, 0, 1, 1, 1, 1] | 0 | 0 |
| [0, 1, 0, 1, 0, 0, 0, 0] | 0 | 0 | [1, 1, 0, 1, 0, 0, 0, 0] | 0 | 0 |
| [0, 1, 0, 1, 0, 0, 0, 1] | 0 | 0 | [1, 1, 0, 1, 0, 0, 0, 1] | 0 | 0 |
| [0, 1, 0, 1, 0, 0, 1, 0] | 0 | 0 | [1, 1, 0, 1, 0, 0, 1, 0] | 0 | 0 |
| [0, 1, 0, 1, 0, 0, 1, 1] | 0 | 0 | [1, 1, 0, 1, 0, 0, 1, 1] | 0 | 0 |
| [0, 1, 0, 1, 0, 1, 0, 0] | 0 | 0 | [1, 1, 0, 1, 0, 1, 0, 0] | 0 | 0 |
| [0, 1, 0, 1, 0, 1, 0, 1] | 57,422,345 | 0.11683 | [1, 1, 0, 1, 0, 1, 0, 1] | 0 | 0 |
| [0, 1, 0, 1, 0, 1, 1, 0] | 0 | 0 | [1, 1, 0, 1, 0, 1, 1, 0] | 0 | 0 |
| [0, 1, 0, 1, 0, 1, 1, 1] | 0 | 0 | [1, 1, 0, 1, 0, 1, 1, 1] | 0 | 0 |
| [0, 1, 0, 1, 1, 0, 0, 0] | 0 | 0 | [1, 1, 0, 1, 1, 0, 0, 0] | 0 | 0 |
| [0, 1, 0, 1, 1, 0, 0, 1] | 0 | 0 | [1, 1, 0, 1, 1, 0, 0, 1] | 0 | 0 |
| [0, 1, 0, 1, 1, 0, 1, 0] | 0 | 0 | [1, 1, 0, 1, 1, 0, 1, 0] | 0 | 0 |
| [0, 1, 0, 1, 1, 0, 1, 1] | 0 | 0 | [1, 1, 0, 1, 1, 0, 1, 1] | 0 | 0 |
| [0, 1, 0, 1, 1, 1, 0, 0] | 0 | 0 | [1, 1, 0, 1, 1, 1, 0, 0] | 0 | 0 |
| [0, 1, 0, 1, 1, 1, 0, 1] | 0 | 0 | [1, 1, 0, 1, 1, 1, 0, 1] | 0 | 0 |
| [0, 1, 0, 1, 1, 1, 1, 0] | 0 | 0 | [1, 1, 0, 1, 1, 1, 1, 0] | 0 | 0 |
| [0, 1, 0, 1, 1, 1, 1, 1] | 0 | 0 | [1, 1, 0, 1, 1, 1, 1, 1] | 0 | 0 |
| [0, 1, 1, 0, 0, 0, 0, 0] | 0 | 0 | [1, 1, 1, 0, 0, 0, 0, 0] | 0 | 0 |
| [0, 1, 1, 0, 0, 0, 0, 1] | 0 | 0 | [1, 1, 1, 0, 0, 0, 0, 1] | 0 | 0 |
| [0, 1, 1, 0, 0, 0, 1, 0] | 0 | 0 | [1, 1, 1, 0, 0, 0, 1, 0] | 0 | 0 |
| [0, 1, 1, 0, 0, 0, 1, 1] | 0 | 0 | [1, 1, 1, 0, 0, 0, 1, 1] | 0 | 0 |
| [0, 1, 1, 0, 0, 1, 0, 0] | 0 | 0 | [1, 1, 1, 0, 0, 1, 0, 0] | 0 | 0 |
| [0, 1, 1, 0, 0, 1, 0, 1] | 0 | 0 | [1, 1, 1, 0, 0, 1, 0, 1] | 0 | 0 |
| [0, 1, 1, 0, 0, 1, 1, 0] | 0 | 0 | [1, 1, 1, 0, 0, 1, 1, 0] | 0 | 0 |
| [0, 1, 1, 0, 0, 1, 1, 1] | 0 | 0 | [1, 1, 1, 0, 0, 1, 1, 1] | 0 | 0 |
| [0, 1, 1, 0, 1, 0, 0, 0] | 0 | 0 | [1, 1, 1, 0, 1, 0, 0, 0] | 0 | 0 |
| [0, 1, 1, 0, 1, 0, 0, 1] | 0 | 0 | [1, 1, 1, 0, 1, 0, 0, 1] | 0 | 0 |
| [0, 1, 1, 0, 1, 0, 1, 0] | 0 | 0 | [1, 1, 1, 0, 1, 0, 1, 0] | 0 | 0 |
| [0, 1, 1, 0, 1, 0, 1, 1] | 0 | 0 | [1, 1, 1, 0, 1, 0, 1, 1] | 0 | 0 |
| [0, 1, 1, 0, 1, 1, 0, 0] | 0 | 0 | [1, 1, 1, 0, 1, 1, 0, 0] | 0 | 0 |

*Continued on next page*

| Spike Pattern | Count | Ratio | Spike Pattern | Count | Ratio |
|---|---|---|---|---|---|
| $[0, 1, 1, 0, 1, 1, 0, 1]$ | 0 | 0 | $[1, 1, 1, 0, 1, 1, 0, 1]$ | 0 | 0 |
| $[0, 1, 1, 0, 1, 1, 1, 0]$ | 0 | 0 | $[1, 1, 1, 0, 1, 1, 1, 0]$ | 0 | 0 |
| $[0, 1, 1, 0, 1, 1, 1, 1]$ | 0 | 0 | $[1, 1, 1, 0, 1, 1, 1, 1]$ | 0 | 0 |
| $[0, 1, 1, 1, 0, 0, 0, 0]$ | 0 | 0 | $[1, 1, 1, 1, 0, 0, 0, 0]$ | 0 | 0 |
| $[0, 1, 1, 1, 0, 0, 0, 1]$ | 0 | 0 | $[1, 1, 1, 1, 0, 0, 0, 1]$ | 0 | 0 |
| $[0, 1, 1, 1, 0, 0, 1, 0]$ | 0 | 0 | $[1, 1, 1, 1, 0, 0, 1, 0]$ | 0 | 0 |
| $[0, 1, 1, 1, 0, 0, 1, 1]$ | 0 | 0 | $[1, 1, 1, 1, 0, 0, 1, 1]$ | 0 | 0 |
| $[0, 1, 1, 1, 0, 1, 0, 0]$ | 0 | 0 | $[1, 1, 1, 1, 0, 1, 0, 0]$ | 0 | 0 |
| $[0, 1, 1, 1, 0, 1, 0, 1]$ | 0 | 0 | $[1, 1, 1, 1, 0, 1, 0, 1]$ | 0 | 0 |
| $[0, 1, 1, 1, 0, 1, 1, 0]$ | 0 | 0 | $[1, 1, 1, 1, 0, 1, 1, 0]$ | 0 | 0 |
| $[0, 1, 1, 1, 0, 1, 1, 1]$ | 0 | 0 | $[1, 1, 1, 1, 0, 1, 1, 1]$ | 0 | 0 |
| $[0, 1, 1, 1, 1, 0, 0, 0]$ | 0 | 0 | $[1, 1, 1, 1, 1, 0, 0, 0]$ | 0 | 0 |
| $[0, 1, 1, 1, 1, 0, 0, 1]$ | 0 | 0 | $[1, 1, 1, 1, 1, 0, 0, 1]$ | 0 | 0 |
| $[0, 1, 1, 1, 1, 0, 1, 0]$ | 0 | 0 | $[1, 1, 1, 1, 1, 0, 1, 0]$ | 0 | 0 |
| $[0, 1, 1, 1, 1, 0, 1, 1]$ | 0 | 0 | $[1, 1, 1, 1, 1, 0, 1, 1]$ | 0 | 0 |
| $[0, 1, 1, 1, 1, 1, 0, 0]$ | 0 | 0 | $[1, 1, 1, 1, 1, 1, 0, 0]$ | 0 | 0 |
| $[0, 1, 1, 1, 1, 1, 0, 1]$ | 0 | 0 | $[1, 1, 1, 1, 1, 1, 0, 1]$ | 0 | 0 |
| $[0, 1, 1, 1, 1, 1, 1, 0]$ | 0 | 0 | $[1, 1, 1, 1, 1, 1, 1, 0]$ | 0 | 0 |
| $[0, 1, 1, 1, 1, 1, 1, 1]$ | 0 | 0 | $[1, 1, 1, 1, 1, 1, 1, 1]$ | 52,494,970 | 0.1068 |
| Spike Entropy | | | 1.6643 | | |
| Firing Rate | | | 0.1905 | | |

Table 16: Distribution of the spike patterns in the encoding layer of Spikformer with direct coding on CIFAR-10 at $T = 8$.

| Spike Pattern | Count | Ratio | Spike Pattern | Count | Ratio |
|---|---|---|---|---|---|
| [0, 0, 0, 0, 0, 0, 0, 0] | 330,957,691 | 0.67334 | [1, 0, 0, 0, 0, 0, 0, 0] | 0 | 0 |
| [0, 0, 0, 0, 0, 0, 0, 1] | 771,824 | 0.00157 | [1, 0, 0, 0, 0, 0, 0, 1] | 0 | 0 |
| [0, 0, 0, 0, 0, 0, 1, 0] | 1,528,431 | 0.00311 | [1, 0, 0, 0, 0, 0, 1, 0] | 0 | 0 |
| [0, 0, 0, 0, 0, 0, 1, 1] | 0 | 0 | [1, 0, 0, 0, 0, 0, 1, 1] | 0 | 0 |
| [0, 0, 0, 0, 0, 1, 0, 0] | 3,246,666 | 0.00660 | [1, 0, 0, 0, 0, 1, 0, 0] | 0 | 0 |
| [0, 0, 0, 0, 0, 1, 0, 1] | 0 | 0 | [1, 0, 0, 0, 0, 1, 0, 1] | 0 | 0 |
| [0, 0, 0, 0, 0, 1, 1, 0] | 0 | 0 | [1, 0, 0, 0, 0, 1, 1, 0] | 0 | 0 |
| [0, 0, 0, 0, 0, 1, 1, 1] | 0 | 0 | [1, 0, 0, 0, 0, 1, 1, 1] | 0 | 0 |
| [0, 0, 0, 0, 1, 0, 0, 0] | 6,402,526 | 0.01303 | [1, 0, 0, 0, 1, 0, 0, 0] | 0 | 0 |
| [0, 0, 0, 0, 1, 0, 0, 1] | 0 | 0 | [1, 0, 0, 0, 1, 0, 0, 1] | 0 | 0 |
| [0, 0, 0, 0, 1, 0, 1, 0] | 0 | 0 | [1, 0, 0, 0, 1, 0, 1, 0] | 0 | 0 |
| [0, 0, 0, 0, 1, 0, 1, 1] | 0 | 0 | [1, 0, 0, 0, 1, 0, 1, 1] | 0 | 0 |
| [0, 0, 0, 0, 1, 1, 0, 0] | 0 | 0 | [1, 0, 0, 0, 1, 1, 0, 0] | 0 | 0 |
| [0, 0, 0, 0, 1, 1, 0, 1] | 0 | 0 | [1, 0, 0, 0, 1, 1, 0, 1] | 0 | 0 |
| [0, 0, 0, 0, 1, 1, 1, 0] | 0 | 0 | [1, 0, 0, 0, 1, 1, 1, 0] | 0 | 0 |
| [0, 0, 0, 0, 1, 1, 1, 1] | 0 | 0 | [1, 0, 0, 0, 1, 1, 1, 1] | 0 | 0 |
| [0, 0, 0, 1, 0, 0, 0, 0] | 0 | 0 | [1, 0, 0, 1, 0, 0, 0, 0] | 0 | 0 |
| [0, 0, 0, 1, 0, 0, 0, 1] | 13,208,866 | 0.02687 | [1, 0, 0, 1, 0, 0, 0, 1] | 0 | 0 |
| [0, 0, 0, 1, 0, 0, 1, 0] | 0 | 0 | [1, 0, 0, 1, 0, 0, 1, 0] | 0 | 0 |
| [0, 0, 0, 1, 0, 0, 1, 1] | 0 | 0 | [1, 0, 0, 1, 0, 0, 1, 1] | 0 | 0 |
| [0, 0, 0, 1, 0, 1, 0, 0] | 0 | 0 | [1, 0, 0, 1, 0, 1, 0, 0] | 0 | 0 |
| [0, 0, 0, 1, 0, 1, 0, 1] | 0 | 0 | [1, 0, 0, 1, 0, 1, 0, 1] | 0 | 0 |
| [0, 0, 0, 1, 0, 1, 1, 0] | 0 | 0 | [1, 0, 0, 1, 0, 1, 1, 0] | 0 | 0 |
| [0, 0, 0, 1, 0, 1, 1, 1] | 0 | 0 | [1, 0, 0, 1, 0, 1, 1, 1] | 0 | 0 |
| [0, 0, 0, 1, 1, 0, 0, 0] | 0 | 0 | [1, 0, 0, 1, 1, 0, 0, 0] | 0 | 0 |
| [0, 0, 0, 1, 1, 0, 0, 1] | 0 | 0 | [1, 0, 0, 1, 1, 0, 0, 1] | 0 | 0 |
| [0, 0, 0, 1, 1, 0, 1, 0] | 0 | 0 | [1, 0, 0, 1, 1, 0, 1, 0] | 0 | 0 |
| [0, 0, 0, 1, 1, 0, 1, 1] | 0 | 0 | [1, 0, 0, 1, 1, 0, 1, 1] | 0 | 0 |
| [0, 0, 0, 1, 1, 1, 0, 0] | 0 | 0 | [1, 0, 0, 1, 1, 1, 0, 0] | 0 | 0 |
| [0, 0, 0, 1, 1, 1, 0, 1] | 0 | 0 | [1, 0, 0, 1, 1, 1, 0, 1] | 0 | 0 |
| [0, 0, 0, 1, 1, 1, 1, 0] | 0 | 0 | [1, 0, 0, 1, 1, 1, 1, 0] | 0 | 0 |
| [0, 0, 0, 1, 1, 1, 1, 1] | 0 | 0 | [1, 0, 0, 1, 1, 1, 1, 1] | 0 | 0 |
| [0, 0, 1, 0, 0, 0, 0, 0] | 0 | 0 | [1, 0, 1, 0, 0, 0, 0, 0] | 0 | 0 |
| [0, 0, 1, 0, 0, 0, 0, 1] | 0 | 0 | [1, 0, 1, 0, 0, 0, 0, 1] | 0 | 0 |
| [0, 0, 1, 0, 0, 0, 1, 0] | 0 | 0 | [1, 0, 1, 0, 0, 0, 1, 0] | 0 | 0 |
| [0, 0, 1, 0, 0, 0, 1, 1] | 0 | 0 | [1, 0, 1, 0, 0, 0, 1, 1] | 0 | 0 |
| [0, 0, 1, 0, 0, 1, 0, 0] | 27,747,968 | 0.05645 | [1, 0, 1, 0, 0, 1, 0, 0] | 0 | 0 |
| [0, 0, 1, 0, 0, 1, 0, 1] | 0 | 0 | [1, 0, 1, 0, 0, 1, 0, 1] | 0 | 0 |
| [0, 0, 1, 0, 0, 1, 1, 0] | 0 | 0 | [1, 0, 1, 0, 0, 1, 1, 0] | 0 | 0 |
| [0, 0, 1, 0, 0, 1, 1, 1] | 0 | 0 | [1, 0, 1, 0, 0, 1, 1, 1] | 0 | 0 |
| [0, 0, 1, 0, 1, 0, 0, 0] | 0 | 0 | [1, 0, 1, 0, 1, 0, 0, 0] | 0 | 0 |
| [0, 0, 1, 0, 1, 0, 0, 1] | 0 | 0 | [1, 0, 1, 0, 1, 0, 0, 1] | 0 | 0 |
| [0, 0, 1, 0, 1, 0, 1, 0] | 0 | 0 | [1, 0, 1, 0, 1, 0, 1, 0] | 0 | 0 |
| [0, 0, 1, 0, 1, 0, 1, 1] | 0 | 0 | [1, 0, 1, 0, 1, 0, 1, 1] | 0 | 0 |
| [0, 0, 1, 0, 1, 1, 0, 0] | 0 | 0 | [1, 0, 1, 0, 1, 1, 0, 0] | 0 | 0 |
| [0, 0, 1, 0, 1, 1, 0, 1] | 0 | 0 | [1, 0, 1, 0, 1, 1, 0, 1] | 0 | 0 |
| [0, 0, 1, 0, 1, 1, 1, 0] | 0 | 0 | [1, 0, 1, 0, 1, 1, 1, 0] | 0 | 0 |
| [0, 0, 1, 0, 1, 1, 1, 1] | 0 | 0 | [1, 0, 1, 0, 1, 1, 1, 1] | 0 | 0 |
| [0, 0, 1, 1, 0, 0, 0, 0] | 0 | 0 | [1, 0, 1, 1, 0, 0, 0, 0] | 0 | 0 |
| [0, 0, 1, 1, 0, 0, 0, 1] | 0 | 0 | [1, 0, 1, 1, 0, 0, 0, 1] | 0 | 0 |
| [0, 0, 1, 1, 0, 0, 1, 0] | 0 | 0 | [1, 0, 1, 1, 0, 0, 1, 0] | 0 | 0 |
| [0, 0, 1, 1, 0, 0, 1, 1] | 0 | 0 | [1, 0, 1, 1, 0, 0, 1, 1] | 0 | 0 |
| [0, 0, 1, 1, 0, 1, 0, 0] | 0 | 0 | [1, 0, 1, 1, 0, 1, 0, 0] | 0 | 0 |
| [0, 0, 1, 1, 0, 1, 0, 1] | 0 | 0 | [1, 0, 1, 1, 0, 1, 0, 1] | 0 | 0 |

*Continued on next page*

| Spike Pattern | Count | Ratio | Spike Pattern | Count | Ratio |
|---|---|---|---|---|---|
| [0, 0, 1, 1, 0, 1, 1, 0] | 0 | 0 | [1, 0, 1, 1, 0, 1, 1, 0] | 0 | 0 |
| [0, 0, 1, 1, 0, 1, 1, 1] | 0 | 0 | [1, 0, 1, 1, 0, 1, 1, 1] | 0 | 0 |
| [0, 0, 1, 1, 1, 0, 0, 0] | 0 | 0 | [1, 0, 1, 1, 1, 0, 0, 0] | 0 | 0 |
| [0, 0, 1, 1, 1, 0, 0, 1] | 0 | 0 | [1, 0, 1, 1, 1, 0, 0, 1] | 0 | 0 |
| [0, 0, 1, 1, 1, 0, 1, 0] | 0 | 0 | [1, 0, 1, 1, 1, 0, 1, 0] | 0 | 0 |
| [0, 0, 1, 1, 1, 0, 1, 1] | 0 | 0 | [1, 0, 1, 1, 1, 0, 1, 1] | 0 | 0 |
| [0, 0, 1, 1, 1, 1, 0, 0] | 0 | 0 | [1, 0, 1, 1, 1, 1, 0, 0] | 0 | 0 |
| [0, 0, 1, 1, 1, 1, 0, 1] | 0 | 0 | [1, 0, 1, 1, 1, 1, 0, 1] | 0 | 0 |
| [0, 0, 1, 1, 1, 1, 1, 0] | 0 | 0 | [1, 0, 1, 1, 1, 1, 1, 0] | 0 | 0 |
| [0, 0, 1, 1, 1, 1, 1, 1] | 0 | 0 | [1, 0, 1, 1, 1, 1, 1, 1] | 0 | 0 |
| [0, 1, 0, 0, 0, 0, 0, 0] | 0 | 0 | [1, 1, 0, 0, 0, 0, 0, 0] | 0 | 0 |
| [0, 1, 0, 0, 0, 0, 0, 1] | 0 | 0 | [1, 1, 0, 0, 0, 0, 0, 1] | 0 | 0 |
| [0, 1, 0, 0, 0, 0, 1, 0] | 0 | 0 | [1, 1, 0, 0, 0, 0, 1, 0] | 0 | 0 |
| [0, 1, 0, 0, 0, 0, 1, 1] | 0 | 0 | [1, 1, 0, 0, 0, 0, 1, 1] | 0 | 0 |
| [0, 1, 0, 0, 0, 1, 0, 0] | 0 | 0 | [1, 1, 0, 0, 0, 1, 0, 0] | 0 | 0 |
| [0, 1, 0, 0, 0, 1, 0, 1] | 0 | 0 | [1, 1, 0, 0, 0, 1, 0, 1] | 0 | 0 |
| [0, 1, 0, 0, 0, 1, 1, 0] | 0 | 0 | [1, 1, 0, 0, 0, 1, 1, 0] | 0 | 0 |
| [0, 1, 0, 0, 0, 1, 1, 1] | 0 | 0 | [1, 1, 0, 0, 0, 1, 1, 1] | 0 | 0 |
| [0, 1, 0, 0, 1, 0, 0, 0] | 0 | 0 | [1, 1, 0, 0, 1, 0, 0, 0] | 0 | 0 |
| [0, 1, 0, 0, 1, 0, 0, 1] | 0 | 0 | [1, 1, 0, 0, 1, 0, 0, 1] | 0 | 0 |
| [0, 1, 0, 0, 1, 0, 1, 0] | 0 | 0 | [1, 1, 0, 0, 1, 0, 1, 0] | 0 | 0 |
| [0, 1, 0, 0, 1, 0, 1, 1] | 0 | 0 | [1, 1, 0, 0, 1, 0, 1, 1] | 0 | 0 |
| [0, 1, 0, 0, 1, 1, 0, 0] | 0 | 0 | [1, 1, 0, 0, 1, 1, 0, 0] | 0 | 0 |
| [0, 1, 0, 0, 1, 1, 0, 1] | 0 | 0 | [1, 1, 0, 0, 1, 1, 0, 1] | 0 | 0 |
| [0, 1, 0, 0, 1, 1, 1, 0] | 0 | 0 | [1, 1, 0, 0, 1, 1, 1, 0] | 0 | 0 |
| [0, 1, 0, 0, 1, 1, 1, 1] | 0 | 0 | [1, 1, 0, 0, 1, 1, 1, 1] | 0 | 0 |
| [0, 1, 0, 1, 0, 0, 0, 0] | 0 | 0 | [1, 1, 0, 1, 0, 0, 0, 0] | 0 | 0 |
| [0, 1, 0, 1, 0, 0, 0, 1] | 0 | 0 | [1, 1, 0, 1, 0, 0, 0, 1] | 0 | 0 |
| [0, 1, 0, 1, 0, 0, 1, 0] | 0 | 0 | [1, 1, 0, 1, 0, 0, 1, 0] | 0 | 0 |
| [0, 1, 0, 1, 0, 0, 1, 1] | 0 | 0 | [1, 1, 0, 1, 0, 0, 1, 1] | 0 | 0 |
| [0, 1, 0, 1, 0, 1, 0, 0] | 0 | 0 | [1, 1, 0, 1, 0, 1, 0, 0] | 0 | 0 |
| [0, 1, 0, 1, 0, 1, 0, 1] | 55,169,205 | 0.11224 | [1, 1, 0, 1, 0, 1, 0, 1] | 0 | 0 |
| [0, 1, 0, 1, 0, 1, 1, 0] | 0 | 0 | [1, 1, 0, 1, 0, 1, 1, 0] | 0 | 0 |
| [0, 1, 0, 1, 0, 1, 1, 1] | 0 | 0 | [1, 1, 0, 1, 0, 1, 1, 1] | 0 | 0 |
| [0, 1, 0, 1, 1, 0, 0, 0] | 0 | 0 | [1, 1, 0, 1, 1, 0, 0, 0] | 0 | 0 |
| [0, 1, 0, 1, 1, 0, 0, 1] | 0 | 0 | [1, 1, 0, 1, 1, 0, 0, 1] | 0 | 0 |
| [0, 1, 0, 1, 1, 0, 1, 0] | 0 | 0 | [1, 1, 0, 1, 1, 0, 1, 0] | 0 | 0 |
| [0, 1, 0, 1, 1, 0, 1, 1] | 0 | 0 | [1, 1, 0, 1, 1, 0, 1, 1] | 0 | 0 |
| [0, 1, 0, 1, 1, 1, 0, 0] | 0 | 0 | [1, 1, 0, 1, 1, 1, 0, 0] | 0 | 0 |
| [0, 1, 0, 1, 1, 1, 0, 1] | 0 | 0 | [1, 1, 0, 1, 1, 1, 0, 1] | 0 | 0 |
| [0, 1, 0, 1, 1, 1, 1, 0] | 0 | 0 | [1, 1, 0, 1, 1, 1, 1, 0] | 0 | 0 |
| [0, 1, 0, 1, 1, 1, 1, 1] | 0 | 0 | [1, 1, 0, 1, 1, 1, 1, 1] | 0 | 0 |
| [0, 1, 1, 0, 0, 0, 0, 0] | 0 | 0 | [1, 1, 1, 0, 0, 0, 0, 0] | 0 | 0 |
| [0, 1, 1, 0, 0, 0, 0, 1] | 0 | 0 | [1, 1, 1, 0, 0, 0, 0, 1] | 0 | 0 |
| [0, 1, 1, 0, 0, 0, 1, 0] | 0 | 0 | [1, 1, 1, 0, 0, 0, 1, 0] | 0 | 0 |
| [0, 1, 1, 0, 0, 0, 1, 1] | 0 | 0 | [1, 1, 1, 0, 0, 0, 1, 1] | 0 | 0 |
| [0, 1, 1, 0, 0, 1, 0, 0] | 0 | 0 | [1, 1, 1, 0, 0, 1, 0, 0] | 0 | 0 |
| [0, 1, 1, 0, 0, 1, 0, 1] | 0 | 0 | [1, 1, 1, 0, 0, 1, 0, 1] | 0 | 0 |
| [0, 1, 1, 0, 0, 1, 1, 0] | 0 | 0 | [1, 1, 1, 0, 0, 1, 1, 0] | 0 | 0 |
| [0, 1, 1, 0, 0, 1, 1, 1] | 0 | 0 | [1, 1, 1, 0, 0, 1, 1, 1] | 0 | 0 |
| [0, 1, 1, 0, 1, 0, 0, 0] | 0 | 0 | [1, 1, 1, 0, 1, 0, 0, 0] | 0 | 0 |
| [0, 1, 1, 0, 1, 0, 0, 1] | 0 | 0 | [1, 1, 1, 0, 1, 0, 0, 1] | 0 | 0 |
| [0, 1, 1, 0, 1, 0, 1, 0] | 0 | 0 | [1, 1, 1, 0, 1, 0, 1, 0] | 0 | 0 |
| [0, 1, 1, 0, 1, 0, 1, 1] | 0 | 0 | [1, 1, 1, 0, 1, 0, 1, 1] | 0 | 0 |
| [0, 1, 1, 0, 1, 1, 0, 0] | 0 | 0 | [1, 1, 1, 0, 1, 1, 0, 0] | 0 | 0 |

*Continued on next page*

| Spike Pattern | Count | Ratio | Spike Pattern | Count | Ratio |
|---|---|---|---|---|---|
| $[0, 1, 1, 0, 1, 1, 0, 1]$ | 0 | 0 | $[1, 1, 1, 0, 1, 1, 0, 1]$ | 0 | 0 |
| $[0, 1, 1, 0, 1, 1, 1, 0]$ | 0 | 0 | $[1, 1, 1, 0, 1, 1, 1, 0]$ | 0 | 0 |
| $[0, 1, 1, 0, 1, 1, 1, 1]$ | 0 | 0 | $[1, 1, 1, 0, 1, 1, 1, 1]$ | 0 | 0 |
| $[0, 1, 1, 1, 0, 0, 0, 0]$ | 0 | 0 | $[1, 1, 1, 1, 0, 0, 0, 0]$ | 0 | 0 |
| $[0, 1, 1, 1, 0, 0, 0, 1]$ | 0 | 0 | $[1, 1, 1, 1, 0, 0, 0, 1]$ | 0 | 0 |
| $[0, 1, 1, 1, 0, 0, 1, 0]$ | 0 | 0 | $[1, 1, 1, 1, 0, 0, 1, 0]$ | 0 | 0 |
| $[0, 1, 1, 1, 0, 0, 1, 1]$ | 0 | 0 | $[1, 1, 1, 1, 0, 0, 1, 1]$ | 0 | 0 |
| $[0, 1, 1, 1, 0, 1, 0, 0]$ | 0 | 0 | $[1, 1, 1, 1, 0, 1, 0, 0]$ | 0 | 0 |
| $[0, 1, 1, 1, 0, 1, 0, 1]$ | 0 | 0 | $[1, 1, 1, 1, 0, 1, 0, 1]$ | 0 | 0 |
| $[0, 1, 1, 1, 0, 1, 1, 0]$ | 0 | 0 | $[1, 1, 1, 1, 0, 1, 1, 0]$ | 0 | 0 |
| $[0, 1, 1, 1, 0, 1, 1, 1]$ | 0 | 0 | $[1, 1, 1, 1, 0, 1, 1, 1]$ | 0 | 0 |
| $[0, 1, 1, 1, 1, 0, 0, 0]$ | 0 | 0 | $[1, 1, 1, 1, 1, 0, 0, 0]$ | 0 | 0 |
| $[0, 1, 1, 1, 1, 0, 0, 1]$ | 0 | 0 | $[1, 1, 1, 1, 1, 0, 0, 1]$ | 0 | 0 |
| $[0, 1, 1, 1, 1, 0, 1, 0]$ | 0 | 0 | $[1, 1, 1, 1, 1, 0, 1, 0]$ | 0 | 0 |
| $[0, 1, 1, 1, 1, 0, 1, 1]$ | 0 | 0 | $[1, 1, 1, 1, 1, 0, 1, 1]$ | 0 | 0 |
| $[0, 1, 1, 1, 1, 1, 0, 0]$ | 0 | 0 | $[1, 1, 1, 1, 1, 1, 0, 0]$ | 0 | 0 |
| $[0, 1, 1, 1, 1, 1, 0, 1]$ | 0 | 0 | $[1, 1, 1, 1, 1, 1, 0, 1]$ | 0 | 0 |
| $[0, 1, 1, 1, 1, 1, 1, 0]$ | 0 | 0 | $[1, 1, 1, 1, 1, 1, 1, 0]$ | 0 | 0 |
| $[0, 1, 1, 1, 1, 1, 1, 1]$ | 0 | 0 | $[1, 1, 1, 1, 1, 1, 1, 1]$ | 52,486,823 | 0.10679 |
| Spike Entropy | | | 1.6272 | | |
| Firing Rate | | | 0.1868 | | |

Table 17: Distribution of the spike patterns in the encoding layer of Spikformer with GAC coding on CIFAR-10 at $T = 8$.

| Spike Pattern | Count | Ratio | Spike Pattern | Count | Ratio |
|---|---|---|---|---|---|
| [0, 0, 0, 0, 0, 0, 0, 0] | 338,033,724 | 0.68773 | [1, 0, 0, 0, 0, 0, 0, 0] | 0 | 0 |
| [0, 0, 0, 0, 0, 0, 0, 1] | 420,120 | 0.00085 | [1, 0, 0, 0, 0, 0, 0, 1] | 0 | 0 |
| [0, 0, 0, 0, 0, 0, 1, 0] | 791,838 | 0.00161 | [1, 0, 0, 0, 0, 0, 1, 0] | 0 | 0 |
| [0, 0, 0, 0, 0, 0, 1, 1] | 0 | 0 | [1, 0, 0, 0, 0, 0, 1, 1] | 0 | 0 |
| [0, 0, 0, 0, 0, 1, 0, 0] | 1,570,624 | 0.00319 | [1, 0, 0, 0, 0, 1, 0, 0] | 0 | 0 |
| [0, 0, 0, 0, 0, 1, 0, 1] | 0 | 0 | [1, 0, 0, 0, 0, 1, 0, 1] | 0 | 0 |
| [0, 0, 0, 0, 0, 1, 1, 0] | 0 | 0 | [1, 0, 0, 0, 0, 1, 1, 0] | 0 | 0 |
| [0, 0, 0, 0, 0, 1, 1, 1] | 0 | 0 | [1, 0, 0, 0, 0, 1, 1, 1] | 0 | 0 |
| [0, 0, 0, 0, 1, 0, 0, 0] | 3,244,095 | 0.00660 | [1, 0, 0, 0, 1, 0, 0, 0] | 0 | 0 |
| [0, 0, 0, 0, 1, 0, 0, 1] | 0 | 0 | [1, 0, 0, 0, 1, 0, 0, 1] | 0 | 0 |
| [0, 0, 0, 0, 1, 0, 1, 0] | 0 | 0 | [1, 0, 0, 0, 1, 0, 1, 0] | 0 | 0 |
| [0, 0, 0, 0, 1, 0, 1, 1] | 0 | 0 | [1, 0, 0, 0, 1, 0, 1, 1] | 0 | 0 |
| [0, 0, 0, 0, 1, 1, 0, 0] | 0 | 0 | [1, 0, 0, 0, 1, 1, 0, 0] | 0 | 0 |
| [0, 0, 0, 0, 1, 1, 0, 1] | 0 | 0 | [1, 0, 0, 0, 1, 1, 0, 1] | 0 | 0 |
| [0, 0, 0, 0, 1, 1, 1, 0] | 0 | 0 | [1, 0, 0, 0, 1, 1, 1, 0] | 0 | 0 |
| [0, 0, 0, 0, 1, 1, 1, 1] | 0 | 0 | [1, 0, 0, 0, 1, 1, 1, 1] | 0 | 0 |
| [0, 0, 0, 1, 0, 0, 0, 0] | 5,826,008 | 0.01185 | [1, 0, 0, 1, 0, 0, 0, 0] | 0 | 0 |
| [0, 0, 0, 1, 0, 0, 0, 1] | 1,168,235 | 0.00238 | [1, 0, 0, 1, 0, 0, 0, 1] | 0 | 0 |
| [0, 0, 0, 1, 0, 0, 1, 0] | 0 | 0 | [1, 0, 0, 1, 0, 0, 1, 0] | 0 | 0 |
| [0, 0, 0, 1, 0, 0, 1, 1] | 0 | 0 | [1, 0, 0, 1, 0, 0, 1, 1] | 0 | 0 |
| [0, 0, 0, 1, 0, 1, 0, 0] | 0 | 0 | [1, 0, 0, 1, 0, 1, 0, 0] | 0 | 0 |
| [0, 0, 0, 1, 0, 1, 0, 1] | 0 | 0 | [1, 0, 0, 1, 0, 1, 0, 1] | 0 | 0 |
| [0, 0, 0, 1, 0, 1, 1, 0] | 0 | 0 | [1, 0, 0, 1, 0, 1, 1, 0] | 0 | 0 |
| [0, 0, 0, 1, 0, 1, 1, 1] | 0 | 0 | [1, 0, 0, 1, 0, 1, 1, 1] | 0 | 0 |
| [0, 0, 0, 1, 1, 0, 0, 0] | 0 | 0 | [1, 0, 0, 1, 1, 0, 0, 0] | 0 | 0 |
| [0, 0, 0, 1, 1, 0, 0, 1] | 0 | 0 | [1, 0, 0, 1, 1, 0, 0, 1] | 0 | 0 |
| [0, 0, 0, 1, 1, 0, 1, 0] | 0 | 0 | [1, 0, 0, 1, 1, 0, 1, 0] | 0 | 0 |
| [0, 0, 0, 1, 1, 0, 1, 1] | 0 | 0 | [1, 0, 0, 1, 1, 0, 1, 1] | 0 | 0 |
| [0, 0, 0, 1, 1, 1, 0, 0] | 0 | 0 | [1, 0, 0, 1, 1, 1, 0, 0] | 0 | 0 |
| [0, 0, 0, 1, 1, 1, 0, 1] | 0 | 0 | [1, 0, 0, 1, 1, 1, 0, 1] | 0 | 0 |
| [0, 0, 0, 1, 1, 1, 1, 0] | 0 | 0 | [1, 0, 0, 1, 1, 1, 1, 0] | 0 | 0 |
| [0, 0, 0, 1, 1, 1, 1, 1] | 0 | 0 | [1, 0, 0, 1, 1, 1, 1, 1] | 0 | 0 |
| [0, 0, 1, 0, 0, 0, 0, 0] | 0 | 0 | [1, 0, 1, 0, 0, 0, 0, 0] | 0 | 0 |
| [0, 0, 1, 0, 0, 0, 0, 1] | 273,521 | 0.00056 | [1, 0, 1, 0, 0, 0, 0, 1] | 0 | 0 |
| [0, 0, 1, 0, 0, 0, 1, 0] | 11,686,870 | 0.02378 | [1, 0, 1, 0, 0, 0, 1, 0] | 0 | 0 |
| [0, 0, 1, 0, 0, 0, 1, 1] | 0 | 0 | [1, 0, 1, 0, 0, 0, 1, 1] | 0 | 0 |
| [0, 0, 1, 0, 0, 1, 0, 0] | 3,856,410 | 0.00785 | [1, 0, 1, 0, 0, 1, 0, 0] | 0 | 0 |
| [0, 0, 1, 0, 0, 1, 0, 1] | 0 | 0 | [1, 0, 1, 0, 0, 1, 0, 1] | 0 | 0 |
| [0, 0, 1, 0, 0, 1, 1, 0] | 0 | 0 | [1, 0, 1, 0, 0, 1, 1, 0] | 0 | 0 |
| [0, 0, 1, 0, 0, 1, 1, 1] | 0 | 0 | [1, 0, 1, 0, 0, 1, 1, 1] | 0 | 0 |
| [0, 0, 1, 0, 1, 0, 0, 0] | 0 | 0 | [1, 0, 1, 0, 1, 0, 0, 0] | 0 | 0 |
| [0, 0, 1, 0, 1, 0, 0, 1] | 0 | 0 | [1, 0, 1, 0, 1, 0, 0, 1] | 0 | 0 |
| [0, 0, 1, 0, 1, 0, 1, 0] | 0 | 0 | [1, 0, 1, 0, 1, 0, 1, 0] | 35,350,352 | 0.07192 |
| [0, 0, 1, 0, 1, 0, 1, 1] | 0 | 0 | [1, 0, 1, 0, 1, 0, 1, 1] | 0 | 0 |
| [0, 0, 1, 0, 1, 1, 0, 0] | 0 | 0 | [1, 0, 1, 0, 1, 1, 0, 0] | 0 | 0 |
| [0, 0, 1, 0, 1, 1, 0, 1] | 0 | 0 | [1, 0, 1, 0, 1, 1, 0, 1] | 0 | 0 |
| [0, 0, 1, 0, 1, 1, 1, 0] | 0 | 0 | [1, 0, 1, 0, 1, 1, 1, 0] | 0 | 0 |
| [0, 0, 1, 0, 1, 1, 1, 1] | 0 | 0 | [1, 0, 1, 0, 1, 1, 1, 1] | 0 | 0 |
| [0, 0, 1, 1, 0, 0, 0, 0] | 0 | 0 | [1, 0, 1, 1, 0, 0, 0, 0] | 0 | 0 |
| [0, 0, 1, 1, 0, 0, 0, 1] | 0 | 0 | [1, 0, 1, 1, 0, 0, 0, 1] | 0 | 0 |
| [0, 0, 1, 1, 0, 0, 1, 0] | 0 | 0 | [1, 0, 1, 1, 0, 0, 1, 0] | 0 | 0 |
| [0, 0, 1, 1, 0, 0, 1, 1] | 0 | 0 | [1, 0, 1, 1, 0, 0, 1, 1] | 0 | 0 |
| [0, 0, 1, 1, 0, 1, 0, 0] | 0 | 0 | [1, 0, 1, 1, 0, 1, 0, 0] | 0 | 0 |
| [0, 0, 1, 1, 0, 1, 0, 1] | 0 | 0 | [1, 0, 1, 1, 0, 1, 0, 1] | 0 | 0 |

*Continued on next page*

| Spike Pattern | Count | Ratio | Spike Pattern | Count | Ratio |
|---|---|---|---|---|---|
| [0, 0, 1, 1, 0, 1, 1, 0] | 0 | 0 | [1, 0, 1, 1, 0, 1, 1, 0] | 0 | 0 |
| [0, 0, 1, 1, 0, 1, 1, 1] | 0 | 0 | [1, 0, 1, 1, 0, 1, 1, 1] | 0 | 0 |
| [0, 0, 1, 1, 1, 0, 0, 0] | 0 | 0 | [1, 0, 1, 1, 1, 0, 0, 0] | 0 | 0 |
| [0, 0, 1, 1, 1, 0, 0, 1] | 0 | 0 | [1, 0, 1, 1, 1, 0, 0, 1] | 0 | 0 |
| [0, 0, 1, 1, 1, 0, 1, 0] | 0 | 0 | [1, 0, 1, 1, 1, 0, 1, 0] | 0 | 0 |
| [0, 0, 1, 1, 1, 0, 1, 1] | 0 | 0 | [1, 0, 1, 1, 1, 0, 1, 1] | 0 | 0 |
| [0, 0, 1, 1, 1, 1, 0, 0] | 0 | 0 | [1, 0, 1, 1, 1, 1, 0, 0] | 0 | 0 |
| [0, 0, 1, 1, 1, 1, 0, 1] | 0 | 0 | [1, 0, 1, 1, 1, 1, 0, 1] | 0 | 0 |
| [0, 0, 1, 1, 1, 1, 1, 0] | 0 | 0 | [1, 0, 1, 1, 1, 1, 1, 0] | 0 | 0 |
| [0, 0, 1, 1, 1, 1, 1, 1] | 0 | 0 | [1, 0, 1, 1, 1, 1, 1, 1] | 0 | 0 |
| [0, 1, 0, 0, 0, 0, 0, 0] | 0 | 0 | [1, 1, 0, 0, 0, 0, 0, 0] | 0 | 0 |
| [0, 1, 0, 0, 0, 0, 0, 1] | 0 | 0 | [1, 1, 0, 0, 0, 0, 0, 1] | 0 | 0 |
| [0, 1, 0, 0, 0, 0, 1, 0] | 0 | 0 | [1, 1, 0, 0, 0, 0, 1, 0] | 0 | 0 |
| [0, 1, 0, 0, 0, 0, 1, 1] | 0 | 0 | [1, 1, 0, 0, 0, 0, 1, 1] | 0 | 0 |
| [0, 1, 0, 0, 0, 1, 0, 0] | 103,065 | 0.00021 | [1, 1, 0, 0, 0, 1, 0, 0] | 0 | 0 |
| [0, 1, 0, 0, 0, 1, 0, 1] | 0 | 0 | [1, 1, 0, 0, 0, 1, 0, 1] | 0 | 0 |
| [0, 1, 0, 0, 0, 1, 1, 0] | 0 | 0 | [1, 1, 0, 0, 0, 1, 1, 0] | 0 | 0 |
| [0, 1, 0, 0, 0, 1, 1, 1] | 0 | 0 | [1, 1, 0, 0, 0, 1, 1, 1] | 0 | 0 |
| [0, 1, 0, 0, 1, 0, 0, 0] | 0 | 0 | [1, 1, 0, 0, 1, 0, 0, 0] | 0 | 0 |
| [0, 1, 0, 0, 1, 0, 0, 1] | 22,682,460 | 0.04615 | [1, 1, 0, 0, 1, 0, 0, 1] | 0 | 0 |
| [0, 1, 0, 0, 1, 0, 1, 0] | 0 | 0 | [1, 1, 0, 0, 1, 0, 1, 0] | 0 | 0 |
| [0, 1, 0, 0, 1, 0, 1, 1] | 0 | 0 | [1, 1, 0, 0, 1, 0, 1, 1] | 0 | 0 |
| [0, 1, 0, 0, 1, 1, 0, 0] | 0 | 0 | [1, 1, 0, 0, 1, 1, 0, 0] | 0 | 0 |
| [0, 1, 0, 0, 1, 1, 0, 1] | 0 | 0 | [1, 1, 0, 0, 1, 1, 0, 1] | 0 | 0 |
| [0, 1, 0, 0, 1, 1, 1, 0] | 0 | 0 | [1, 1, 0, 0, 1, 1, 1, 0] | 0 | 0 |
| [0, 1, 0, 0, 1, 1, 1, 1] | 0 | 0 | [1, 1, 0, 0, 1, 1, 1, 1] | 0 | 0 |
| [0, 1, 0, 1, 0, 0, 0, 0] | 0 | 0 | [1, 1, 0, 1, 0, 0, 0, 0] | 0 | 0 |
| [0, 1, 0, 1, 0, 0, 0, 1] | 0 | 0 | [1, 1, 0, 1, 0, 0, 0, 1] | 0 | 0 |
| [0, 1, 0, 1, 0, 0, 1, 0] | 0 | 0 | [1, 1, 0, 1, 0, 0, 1, 0] | 0 | 0 |
| [0, 1, 0, 1, 0, 0, 1, 1] | 0 | 0 | [1, 1, 0, 1, 0, 0, 1, 1] | 0 | 0 |
| [0, 1, 0, 1, 0, 1, 0, 0] | 0 | 0 | [1, 1, 0, 1, 0, 1, 0, 0] | 0 | 0 |
| [0, 1, 0, 1, 0, 1, 0, 1] | 17,535,536 | 0.03568 | [1, 1, 0, 1, 0, 1, 0, 1] | 0 | 0 |
| [0, 1, 0, 1, 0, 1, 1, 0] | 0 | 0 | [1, 1, 0, 1, 0, 1, 1, 0] | 0 | 0 |
| [0, 1, 0, 1, 0, 1, 1, 1] | 0 | 0 | [1, 1, 0, 1, 0, 1, 1, 1] | 0 | 0 |
| [0, 1, 0, 1, 1, 0, 0, 0] | 0 | 0 | [1, 1, 0, 1, 1, 0, 0, 0] | 0 | 0 |
| [0, 1, 0, 1, 1, 0, 0, 1] | 0 | 0 | [1, 1, 0, 1, 1, 0, 0, 1] | 0 | 0 |
| [0, 1, 0, 1, 1, 0, 1, 0] | 0 | 0 | [1, 1, 0, 1, 1, 0, 1, 0] | 0 | 0 |
| [0, 1, 0, 1, 1, 0, 1, 1] | 0 | 0 | [1, 1, 0, 1, 1, 0, 1, 1] | 0 | 0 |
| [0, 1, 0, 1, 1, 1, 0, 0] | 0 | 0 | [1, 1, 0, 1, 1, 1, 0, 0] | 0 | 0 |
| [0, 1, 0, 1, 1, 1, 0, 1] | 0 | 0 | [1, 1, 0, 1, 1, 1, 0, 1] | 0 | 0 |
| [0, 1, 0, 1, 1, 1, 1, 0] | 0 | 0 | [1, 1, 0, 1, 1, 1, 1, 0] | 0 | 0 |
| [0, 1, 0, 1, 1, 1, 1, 1] | 0 | 0 | [1, 1, 0, 1, 1, 1, 1, 1] | 0 | 0 |
| [0, 1, 1, 0, 0, 0, 0, 0] | 0 | 0 | [1, 1, 1, 0, 0, 0, 0, 0] | 0 | 0 |
| [0, 1, 1, 0, 0, 0, 0, 1] | 0 | 0 | [1, 1, 1, 0, 0, 0, 0, 1] | 0 | 0 |
| [0, 1, 1, 0, 0, 0, 1, 0] | 0 | 0 | [1, 1, 1, 0, 0, 0, 1, 0] | 0 | 0 |
| [0, 1, 1, 0, 0, 0, 1, 1] | 0 | 0 | [1, 1, 1, 0, 0, 0, 1, 1] | 0 | 0 |
| [0, 1, 1, 0, 0, 1, 0, 0] | 0 | 0 | [1, 1, 1, 0, 0, 1, 0, 0] | 0 | 0 |
| [0, 1, 1, 0, 0, 1, 0, 1] | 0 | 0 | [1, 1, 1, 0, 0, 1, 0, 1] | 0 | 0 |
| [0, 1, 1, 0, 0, 1, 1, 0] | 0 | 0 | [1, 1, 1, 0, 0, 1, 1, 0] | 0 | 0 |
| [0, 1, 1, 0, 0, 1, 1, 1] | 0 | 0 | [1, 1, 1, 0, 0, 1, 1, 1] | 0 | 0 |
| [0, 1, 1, 0, 1, 0, 0, 0] | 0 | 0 | [1, 1, 1, 0, 1, 0, 0, 0] | 0 | 0 |
| [0, 1, 1, 0, 1, 0, 0, 1] | 0 | 0 | [1, 1, 1, 0, 1, 0, 0, 1] | 0 | 0 |
| [0, 1, 1, 0, 1, 0, 1, 0] | 0 | 0 | [1, 1, 1, 0, 1, 0, 1, 0] | 0 | 0 |
| [0, 1, 1, 0, 1, 0, 1, 1] | 0 | 0 | [1, 1, 1, 0, 1, 0, 1, 1] | 0 | 0 |
| [0, 1, 1, 0, 1, 1, 0, 0] | 0 | 0 | [1, 1, 1, 0, 1, 1, 0, 0] | 0 | 0 |

*Continued on next page*

| Spike Pattern | Count | Ratio | Spike Pattern | Count | Ratio |
|---|---|---|---|---|---|
| $[0,1,1,0,1,1,0,1]$ | 0 | 0 | $[1,1,1,0,1,1,0,1]$ | 0 | 0 |
| $[0,1,1,0,1,1,1,0]$ | 0 | 0 | $[1,1,1,0,1,1,1,0]$ | 0 | 0 |
| $[0,1,1,0,1,1,1,1]$ | 0 | 0 | $[1,1,1,0,1,1,1,1]$ | 0 | 0 |
| $[0,1,1,1,0,0,0,0]$ | 0 | 0 | $[1,1,1,1,0,0,0,0]$ | 0 | 0 |
| $[0,1,1,1,0,0,0,1]$ | 0 | 0 | $[1,1,1,1,0,0,0,1]$ | 0 | 0 |
| $[0,1,1,1,0,0,1,0]$ | 0 | 0 | $[1,1,1,1,0,0,1,0]$ | 0 | 0 |
| $[0,1,1,1,0,0,1,1]$ | 0 | 0 | $[1,1,1,1,0,0,1,1]$ | 0 | 0 |
| $[0,1,1,1,0,1,0,0]$ | 0 | 0 | $[1,1,1,1,0,1,0,0]$ | 0 | 0 |
| $[0,1,1,1,0,1,0,1]$ | 0 | 0 | $[1,1,1,1,0,1,0,1]$ | 0 | 0 |
| $[0,1,1,1,0,1,1,0]$ | 0 | 0 | $[1,1,1,1,0,1,1,0]$ | 0 | 0 |
| $[0,1,1,1,0,1,1,1]$ | 0 | 0 | $[1,1,1,1,0,1,1,1]$ | 0 | 0 |
| $[0,1,1,1,1,0,0,0]$ | 0 | 0 | $[1,1,1,1,1,0,0,0]$ | 0 | 0 |
| $[0,1,1,1,1,0,0,1]$ | 0 | 0 | $[1,1,1,1,1,0,0,1]$ | 0 | 0 |
| $[0,1,1,1,1,0,1,0]$ | 0 | 0 | $[1,1,1,1,1,0,1,0]$ | 0 | 0 |
| $[0,1,1,1,1,0,1,1]$ | 0 | 0 | $[1,1,1,1,1,0,1,1]$ | 0 | 0 |
| $[0,1,1,1,1,1,0,0]$ | 0 | 0 | $[1,1,1,1,1,1,0,0]$ | 0 | 0 |
| $[0,1,1,1,1,1,0,1]$ | 0 | 0 | $[1,1,1,1,1,1,0,1]$ | 0 | 0 |
| $[0,1,1,1,1,1,1,0]$ | 0 | 0 | $[1,1,1,1,1,1,1,0]$ | 0 | 0 |
| $[0,1,1,1,1,1,1,1]$ | 0 | 0 | $[1,1,1,1,1,1,1,1]$ | 48,977,142 | 0.09964 |
| Spike Entropy | | | 1.7386 | | |
| Firing Rate | | | 0.1825 | | |

Table 18: Distribution of the spike patterns in the encoding layer of Spikformer with IMP coding on CIFAR-10 at $T = 8$.

| Spike Pattern | Count | Ratio | Spike Pattern | Count | Ratio |
|---|---|---|---|---|---|
| [0, 0, 0, 0, 0, 0, 0, 0] | 166,978,088 | 0.33972 | [1, 0, 0, 0, 0, 0, 0, 0] | 9,513,446 | 0.01936 |
| [0, 0, 0, 0, 0, 0, 0, 1] | 8,830,253 | 0.01796 | [1, 0, 0, 0, 0, 0, 0, 1] | 392,394 | 0.00080 |
| [0, 0, 0, 0, 0, 0, 1, 0] | 8,802,154 | 0.01791 | [1, 0, 0, 0, 0, 0, 1, 0] | 2,181,415 | 0.00444 |
| [0, 0, 0, 0, 0, 0, 1, 1] | 924,376 | 0.00188 | [1, 0, 0, 0, 0, 0, 1, 1] | 135,224 | 0.00028 |
| [0, 0, 0, 0, 0, 1, 0, 0] | 10,439,976 | 0.02124 | [1, 0, 0, 0, 0, 1, 0, 0] | 418,115 | 0.00085 |
| [0, 0, 0, 0, 0, 1, 0, 1] | 6,276,028 | 0.01277 | [1, 0, 0, 0, 0, 1, 0, 1] | 230,261 | 0.00047 |
| [0, 0, 0, 0, 0, 1, 1, 0] | 707,642 | 0.00144 | [1, 0, 0, 0, 0, 1, 1, 0] | 109,016 | 0.00022 |
| [0, 0, 0, 0, 0, 1, 1, 1] | 654,040 | 0.00133 | [1, 0, 0, 0, 0, 1, 1, 1] | 80,885 | 0.00016 |
| [0, 0, 0, 0, 1, 0, 0, 0] | 10,414,246 | 0.02119 | [1, 0, 0, 0, 1, 0, 0, 0] | 1,152,106 | 0.00234 |
| [0, 0, 0, 0, 1, 0, 0, 1] | 709,126 | 0.00144 | [1, 0, 0, 0, 1, 0, 0, 1] | 60,478 | 0.00012 |
| [0, 0, 0, 0, 1, 0, 1, 0] | 6,254,257 | 0.01272 | [1, 0, 0, 0, 1, 0, 1, 0] | 1,728,587 | 0.00352 |
| [0, 0, 0, 0, 1, 0, 1, 1] | 653,259 | 0.00133 | [1, 0, 0, 0, 1, 0, 1, 1] | 133,119 | 0.00027 |
| [0, 0, 0, 0, 1, 1, 0, 0] | 1,055,761 | 0.00215 | [1, 0, 0, 0, 1, 1, 0, 0] | 74,482 | 0.00015 |
| [0, 0, 0, 0, 1, 1, 0, 1] | 611,561 | 0.00124 | [1, 0, 0, 0, 1, 1, 0, 1] | 42,115 | 0.00009 |
| [0, 0, 0, 0, 1, 1, 1, 0] | 608,929 | 0.00124 | [1, 0, 0, 0, 1, 1, 1, 0] | 112,564 | 0.00023 |
| [0, 0, 0, 0, 1, 1, 1, 1] | 569,225 | 0.00116 | [1, 0, 0, 0, 1, 1, 1, 1] | 96,101 | 0.00020 |
| [0, 0, 0, 1, 0, 0, 0, 0] | 13,875,066 | 0.02823 | [1, 0, 0, 1, 0, 0, 0, 0] | 801,618 | 0.00163 |
| [0, 0, 0, 1, 0, 0, 0, 1] | 2,203,497 | 0.00448 | [1, 0, 0, 1, 0, 0, 0, 1] | 96,118 | 0.00020 |
| [0, 0, 0, 1, 0, 0, 1, 0] | 586,408 | 0.00119 | [1, 0, 0, 1, 0, 0, 1, 0] | 133,181 | 0.00027 |
| [0, 0, 0, 1, 0, 0, 1, 1] | 155,802 | 0.00032 | [1, 0, 0, 1, 0, 0, 1, 1] | 26,500 | 0.00005 |
| [0, 0, 0, 1, 0, 1, 0, 0] | 8,315,241 | 0.01692 | [1, 0, 0, 1, 0, 1, 0, 0] | 357,330 | 0.00073 |
| [0, 0, 0, 1, 0, 1, 0, 1] | 11,461,260 | 0.02332 | [1, 0, 0, 1, 0, 1, 0, 1] | 378,856 | 0.00077 |
| [0, 0, 0, 1, 0, 1, 1, 0] | 433,513 | 0.00088 | [1, 0, 0, 1, 0, 1, 1, 0] | 71,315 | 0.00015 |
| [0, 0, 0, 1, 0, 1, 1, 1] | 860,104 | 0.00175 | [1, 0, 0, 1, 0, 1, 1, 1] | 105,466 | 0.00021 |
| [0, 0, 0, 1, 1, 0, 0, 0] | 883,826 | 0.00180 | [1, 0, 0, 1, 1, 0, 0, 0] | 87,782 | 0.00018 |
| [0, 0, 0, 1, 1, 0, 0, 1] | 167,854 | 0.00034 | [1, 0, 0, 1, 1, 0, 0, 1] | 13,783 | 0.00003 |
| [0, 0, 0, 1, 1, 0, 1, 0] | 405,627 | 0.00082 | [1, 0, 0, 1, 1, 0, 1, 0] | 99,569 | 0.00020 |
| [0, 0, 0, 1, 1, 0, 1, 1] | 108,798 | 0.00022 | [1, 0, 0, 1, 1, 0, 1, 1] | 22,741 | 0.00005 |
| [0, 0, 0, 1, 1, 1, 0, 0] | 755,319 | 0.00154 | [1, 0, 0, 1, 1, 1, 0, 0] | 55,661 | 0.00011 |
| [0, 0, 0, 1, 1, 1, 0, 1] | 1,068,954 | 0.00217 | [1, 0, 0, 1, 1, 1, 0, 1] | 67,964 | 0.00014 |
| [0, 0, 0, 1, 1, 1, 1, 0] | 359,435 | 0.00073 | [1, 0, 0, 1, 1, 1, 1, 0] | 69,454 | 0.00014 |
| [0, 0, 0, 1, 1, 1, 1, 1] | 744,798 | 0.00152 | [1, 0, 0, 1, 1, 1, 1, 1] | 115,930 | 0.00024 |
| [0, 0, 1, 0, 0, 0, 0, 0] | 13,875,540 | 0.02823 | [1, 0, 1, 0, 0, 0, 0, 0] | 5,314,878 | 0.01081 |
| [0, 0, 1, 0, 0, 0, 0, 1] | 586,328 | 0.00119 | [1, 0, 1, 0, 0, 0, 0, 1] | 165,056 | 0.00034 |
| [0, 0, 1, 0, 0, 0, 1, 0] | 2,202,679 | 0.00448 | [1, 0, 1, 0, 0, 0, 1, 0] | 1,868,819 | 0.00380 |
| [0, 0, 1, 0, 0, 0, 1, 1] | 155,493 | 0.00032 | [1, 0, 1, 0, 0, 0, 1, 1] | 86,177 | 0.00017 |
| [0, 0, 1, 0, 0, 1, 0, 0] | 885,163 | 0.00180 | [1, 0, 1, 0, 0, 1, 0, 0] | 230,771 | 0.00047 |
| [0, 0, 1, 0, 0, 1, 0, 1] | 404,652 | 0.00082 | [1, 0, 1, 0, 0, 1, 0, 1] | 100,306 | 0.00020 |
| [0, 0, 1, 0, 0, 1, 1, 0] | 167,824 | 0.00034 | [1, 0, 1, 0, 0, 1, 1, 0] | 90,448 | 0.00018 |
| [0, 0, 1, 0, 0, 1, 1, 1] | 108,576 | 0.00022 | [1, 0, 1, 0, 0, 1, 1, 1] | 50,985 | 0.00010 |
| [0, 0, 1, 0, 1, 0, 0, 0] | 8,283,191 | 0.01685 | [1, 0, 1, 0, 1, 0, 0, 0] | 3,759,113 | 0.00765 |
| [0, 0, 1, 0, 1, 0, 0, 1] | 434,009 | 0.00088 | [1, 0, 1, 0, 1, 0, 0, 1] | 150,195 | 0.00031 |
| [0, 0, 1, 0, 1, 0, 1, 0] | 11,461,617 | 0.02332 | [1, 0, 1, 0, 1, 0, 1, 0] | 25,557,536 | 0.05200 |
| [0, 0, 1, 0, 1, 0, 1, 1] | 863,192 | 0.00176 | [1, 0, 1, 0, 1, 0, 1, 1] | 1,423,576 | 0.00290 |
| [0, 0, 1, 0, 1, 1, 0, 0] | 754,439 | 0.00153 | [1, 0, 1, 0, 1, 1, 0, 0] | 236,823 | 0.00048 |
| [0, 0, 1, 0, 1, 1, 0, 1] | 358,953 | 0.00073 | [1, 0, 1, 0, 1, 1, 0, 1] | 105,855 | 0.00021 |
| [0, 0, 1, 0, 1, 1, 1, 0] | 1,070,523 | 0.00218 | [1, 0, 1, 0, 1, 1, 1, 0] | 1,705,014 | 0.00347 |
| [0, 0, 1, 0, 1, 1, 1, 1] | 749,485 | 0.00153 | [1, 0, 1, 0, 1, 1, 1, 1] | 1,076,246 | 0.00219 |
| [0, 0, 1, 1, 0, 0, 0, 0] | 2,069,223 | 0.00421 | [1, 0, 1, 1, 0, 0, 0, 0] | 619,136 | 0.00126 |
| [0, 0, 1, 1, 0, 0, 0, 1] | 246,054 | 0.00050 | [1, 0, 1, 1, 0, 0, 0, 1] | 59,275 | 0.00012 |
| [0, 0, 1, 1, 0, 0, 1, 0] | 246,872 | 0.00050 | [1, 0, 1, 1, 0, 0, 1, 0] | 174,810 | 0.00036 |
| [0, 0, 1, 1, 0, 0, 1, 1] | 51,835 | 0.00011 | [1, 0, 1, 1, 0, 0, 1, 1] | 26,124 | 0.00005 |
| [0, 0, 1, 1, 0, 1, 0, 0] | 1,162,307 | 0.00236 | [1, 0, 1, 1, 0, 1, 0, 0] | 264,551 | 0.00054 |
| [0, 0, 1, 1, 0, 1, 0, 1] | 1,138,064 | 0.00231 | [1, 0, 1, 1, 0, 1, 0, 1] | 228,051 | 0.00046 |

*Continued on next page*

| Spike Pattern | Count | Ratio | Spike Pattern | Count | Ratio |
|---|---|---|---|---|---|
| [0, 0, 1, 1, 0, 1, 1, 0] | 173,135 | 0.00035 | [1, 0, 1, 1, 0, 1, 1, 0] | 86,136 | 0.00017 |
| [0, 0, 1, 1, 0, 1, 1, 1] | 258,765 | 0.00053 | [1, 0, 1, 1, 0, 1, 1, 1] | 99,880 | 0.00020 |
| [0, 0, 1, 1, 1, 0, 0, 0] | 1,156,988 | 0.00235 | [1, 0, 1, 1, 1, 0, 0, 0] | 403,385 | 0.00082 |
| [0, 0, 1, 1, 1, 0, 0, 1] | 172,341 | 0.00035 | [1, 0, 1, 1, 1, 0, 0, 1] | 50,620 | 0.00010 |
| [0, 0, 1, 1, 1, 0, 1, 0] | 1,139,849 | 0.00232 | [1, 0, 1, 1, 1, 0, 1, 0] | 2,158,541 | 0.00439 |
| [0, 0, 1, 1, 1, 0, 1, 1] | 260,298 | 0.00053 | [1, 0, 1, 1, 1, 0, 1, 1] | 413,268 | 0.00084 |
| [0, 0, 1, 1, 1, 1, 0, 0] | 938,898 | 0.00191 | [1, 0, 1, 1, 1, 1, 0, 0] | 256,378 | 0.00052 |
| [0, 0, 1, 1, 1, 1, 0, 1] | 1,051,950 | 0.00214 | [1, 0, 1, 1, 1, 1, 0, 1] | 249,442 | 0.00051 |
| [0, 0, 1, 1, 1, 1, 1, 0] | 1,053,394 | 0.00214 | [1, 0, 1, 1, 1, 1, 1, 0] | 1,597,605 | 0.00325 |
| [0, 0, 1, 1, 1, 1, 1, 1] | 1,832,734 | 0.00373 | [1, 0, 1, 1, 1, 1, 1, 1] | 2,463,570 | 0.00501 |
| [0, 1, 0, 0, 0, 0, 0, 0] | 9,590,581 | 0.01951 | [1, 1, 0, 0, 0, 0, 0, 0] | 1,647,164 | 0.00335 |
| [0, 1, 0, 0, 0, 0, 0, 1] | 2,226,551 | 0.00453 | [1, 1, 0, 0, 0, 0, 0, 1] | 340,639 | 0.00069 |
| [0, 1, 0, 0, 0, 0, 1, 0] | 397,399 | 0.00081 | [1, 1, 0, 0, 0, 0, 1, 0] | 342,632 | 0.00070 |
| [0, 1, 0, 0, 0, 0, 1, 1] | 137,468 | 0.00028 | [1, 1, 0, 0, 0, 0, 1, 1] | 101,762 | 0.00021 |
| [0, 1, 0, 0, 0, 1, 0, 0] | 1,172,184 | 0.00238 | [1, 1, 0, 0, 0, 1, 0, 0] | 157,183 | 0.00032 |
| [0, 1, 0, 0, 0, 1, 0, 1] | 1,748,051 | 0.00356 | [1, 1, 0, 0, 0, 1, 0, 1] | 196,883 | 0.00040 |
| [0, 1, 0, 0, 0, 1, 1, 0] | 61,588 | 0.00013 | [1, 1, 0, 0, 0, 1, 1, 0] | 36,292 | 0.00007 |
| [0, 1, 0, 0, 0, 1, 1, 1] | 133,859 | 0.00027 | [1, 1, 0, 0, 0, 1, 1, 1] | 60,848 | 0.00012 |
| [0, 1, 0, 0, 1, 0, 0, 0] | 425,154 | 0.00086 | [1, 1, 0, 0, 1, 0, 0, 0] | 156,747 | 0.00032 |
| [0, 1, 0, 0, 1, 0, 0, 1] | 112,041 | 0.00023 | [1, 1, 0, 0, 1, 0, 0, 1] | 36,216 | 0.00007 |
| [0, 1, 0, 0, 1, 0, 1, 0] | 233,155 | 0.00047 | [1, 1, 0, 0, 1, 0, 1, 0] | 196,911 | 0.00040 |
| [0, 1, 0, 0, 1, 0, 1, 1] | 81,906 | 0.00017 | [1, 1, 0, 0, 1, 0, 1, 1] | 61,451 | 0.00013 |
| [0, 1, 0, 0, 1, 1, 0, 0] | 75,695 | 0.00015 | [1, 1, 0, 0, 1, 1, 0, 0] | 22,643 | 0.00005 |
| [0, 1, 0, 0, 1, 1, 0, 1] | 114,457 | 0.00023 | [1, 1, 0, 0, 1, 1, 0, 1] | 28,090 | 0.00006 |
| [0, 1, 0, 0, 1, 1, 1, 0] | 43,172 | 0.00009 | [1, 1, 0, 0, 1, 1, 1, 0] | 27,892 | 0.00006 |
| [0, 1, 0, 0, 1, 1, 1, 1] | 96,608 | 0.00020 | [1, 1, 0, 0, 1, 1, 1, 1] | 51,863 | 0.00011 |
| [0, 1, 0, 1, 0, 0, 0, 0] | 5,357,109 | 0.01090 | [1, 1, 0, 1, 0, 0, 0, 0] | 736,347 | 0.00150 |
| [0, 1, 0, 1, 0, 0, 0, 1] | 1,897,437 | 0.00386 | [1, 1, 0, 1, 0, 0, 0, 1] | 247,622 | 0.00050 |
| [0, 1, 0, 1, 0, 0, 1, 0] | 168,450 | 0.00034 | [1, 1, 0, 1, 0, 0, 1, 0] | 113,743 | 0.00023 |
| [0, 1, 0, 1, 0, 0, 1, 1] | 86,691 | 0.00018 | [1, 1, 0, 1, 0, 0, 1, 1] | 55,728 | 0.00011 |
| [0, 1, 0, 1, 0, 1, 0, 0] | 3,782,721 | 0.00770 | [1, 1, 0, 1, 0, 1, 0, 0] | 399,293 | 0.00081 |
| [0, 1, 0, 1, 0, 1, 0, 1] | 25,384,806 | 0.05165 | [1, 1, 0, 1, 0, 1, 0, 1] | 1,931,294 | 0.00393 |
| [0, 1, 0, 1, 0, 1, 1, 0] | 151,732 | 0.00031 | [1, 1, 0, 1, 0, 1, 1, 0] | 72,079 | 0.00015 |
| [0, 1, 0, 1, 0, 1, 1, 1] | 1,418,875 | 0.00289 | [1, 1, 0, 1, 0, 1, 1, 1] | 460,687 | 0.00094 |
| [0, 1, 0, 1, 1, 0, 0, 0] | 235,228 | 0.00048 | [1, 1, 0, 1, 1, 0, 0, 0] | 68,648 | 0.00014 |
| [0, 1, 0, 1, 1, 0, 0, 1] | 92,351 | 0.00019 | [1, 1, 0, 1, 1, 0, 0, 1] | 25,366 | 0.00005 |
| [0, 1, 0, 1, 1, 0, 1, 0] | 102,671 | 0.00021 | [1, 1, 0, 1, 1, 0, 1, 0] | 67,715 | 0.00014 |
| [0, 1, 0, 1, 1, 0, 1, 1] | 51,490 | 0.00011 | [1, 1, 0, 1, 1, 0, 1, 1] | 33,684 | 0.00007 |
| [0, 1, 0, 1, 1, 1, 0, 0] | 239,042 | 0.00049 | [1, 1, 0, 1, 1, 1, 0, 0] | 53,849 | 0.00011 |
| [0, 1, 0, 1, 1, 1, 0, 1] | 1,699,280 | 0.00346 | [1, 1, 0, 1, 1, 1, 0, 1] | 284,509 | 0.00058 |
| [0, 1, 0, 1, 1, 1, 1, 0] | 107,626 | 0.00022 | [1, 1, 0, 1, 1, 1, 1, 0] | 54,865 | 0.00011 |
| [0, 1, 0, 1, 1, 1, 1, 1] | 1,071,170 | 0.00218 | [1, 1, 0, 1, 1, 1, 1, 1] | 405,608 | 0.00082 |
| [0, 1, 1, 0, 0, 0, 0, 0] | 805,300 | 0.00164 | [1, 1, 1, 0, 0, 0, 0, 0] | 735,791 | 0.00150 |
| [0, 1, 1, 0, 0, 0, 0, 1] | 137,191 | 0.00028 | [1, 1, 1, 0, 0, 0, 0, 1] | 114,502 | 0.00023 |
| [0, 1, 1, 0, 0, 0, 1, 0] | 98,351 | 0.00020 | [1, 1, 1, 0, 0, 0, 1, 0] | 245,772 | 0.00050 |
| [0, 1, 1, 0, 0, 0, 1, 1] | 27,141 | 0.00006 | [1, 1, 1, 0, 0, 0, 1, 1] | 55,104 | 0.00011 |
| [0, 1, 1, 0, 0, 1, 0, 0] | 89,126 | 0.00018 | [1, 1, 1, 0, 0, 1, 0, 0] | 68,869 | 0.00014 |
| [0, 1, 1, 0, 0, 1, 0, 1] | 100,748 | 0.00020 | [1, 1, 1, 0, 0, 1, 0, 1] | 67,376 | 0.00014 |
| [0, 1, 1, 0, 0, 1, 1, 0] | 14,038 | 0.00003 | [1, 1, 1, 0, 0, 1, 1, 0] | 25,216 | 0.00005 |
| [0, 1, 1, 0, 0, 1, 1, 1] | 22,889 | 0.00005 | [1, 1, 1, 0, 0, 1, 1, 1] | 33,126 | 0.00007 |
| [0, 1, 1, 0, 1, 0, 0, 0] | 359,617 | 0.00073 | [1, 1, 1, 0, 1, 0, 0, 0] | 396,169 | 0.00081 |
| [0, 1, 1, 0, 1, 0, 0, 1] | 72,902 | 0.00015 | [1, 1, 1, 0, 1, 0, 0, 1] | 71,954 | 0.00015 |
| [0, 1, 1, 0, 1, 0, 1, 0] | 383,809 | 0.00078 | [1, 1, 1, 0, 1, 0, 1, 0] | 1,940,450 | 0.00395 |
| [0, 1, 1, 0, 1, 0, 1, 1] | 107,570 | 0.00022 | [1, 1, 1, 0, 1, 0, 1, 1] | 463,704 | 0.00094 |
| [0, 1, 1, 0, 1, 1, 0, 0] | 56,599 | 0.00012 | [1, 1, 1, 0, 1, 1, 0, 0] | 53,706 | 0.00011 |

*Continued on next page*

| Spike Pattern | Count | Ratio | Spike Pattern | Count | Ratio |
|---|---|---|---|---|---|
| $[0, 1, 1, 0, 1, 1, 0, 1]$ | 69,347 | 0.00014 | $[1, 1, 1, 0, 1, 1, 0, 1]$ | 55,115 | 0.00011 |
| $[0, 1, 1, 0, 1, 1, 1, 0]$ | 68,691 | 0.00014 | $[1, 1, 1, 0, 1, 1, 1, 0]$ | 288,965 | 0.00059 |
| $[0, 1, 1, 0, 1, 1, 1, 1]$ | 117,212 | 0.00024 | $[1, 1, 1, 0, 1, 1, 1, 1]$ | 410,063 | 0.00083 |
| $[0, 1, 1, 1, 0, 0, 0, 0]$ | 626,320 | 0.00127 | $[1, 1, 1, 1, 0, 0, 0, 0]$ | 524,667 | 0.00107 |
| $[0, 1, 1, 1, 0, 0, 0, 1]$ | 176,202 | 0.00036 | $[1, 1, 1, 1, 0, 0, 0, 1]$ | 141,241 | 0.00029 |
| $[0, 1, 1, 1, 0, 0, 1, 0]$ | 60,238 | 0.00012 | $[1, 1, 1, 1, 0, 0, 1, 0]$ | 140,653 | 0.00029 |
| $[0, 1, 1, 1, 0, 0, 1, 1]$ | 26,423 | 0.00005 | $[1, 1, 1, 1, 0, 0, 1, 1]$ | 53,288 | 0.00011 |
| $[0, 1, 1, 1, 0, 1, 0, 0]$ | 407,982 | 0.00083 | $[1, 1, 1, 1, 0, 1, 0, 0]$ | 282,270 | 0.00057 |
| $[0, 1, 1, 1, 0, 1, 0, 1]$ | 2,151,062 | 0.00438 | $[1, 1, 1, 1, 0, 1, 0, 1]$ | 1,174,816 | 0.00239 |
| $[0, 1, 1, 1, 0, 1, 1, 0]$ | 51,179 | 0.00010 | $[1, 1, 1, 1, 0, 1, 1, 0]$ | 83,582 | 0.00017 |
| $[0, 1, 1, 1, 0, 1, 1, 1]$ | 411,145 | 0.00084 | $[1, 1, 1, 1, 0, 1, 1, 1]$ | 456,045 | 0.00093 |
| $[0, 1, 1, 1, 1, 0, 0, 0]$ | 270,206 | 0.00055 | $[1, 1, 1, 1, 1, 0, 0, 0]$ | 282,787 | 0.00057 |
| $[0, 1, 1, 1, 1, 0, 0, 1]$ | 87,441 | 0.00018 | $[1, 1, 1, 1, 1, 0, 0, 1]$ | 83,519 | 0.00017 |
| $[0, 1, 1, 1, 1, 0, 1, 0]$ | 231,147 | 0.00047 | $[1, 1, 1, 1, 1, 0, 1, 0]$ | 1,183,180 | 0.00241 |
| $[0, 1, 1, 1, 1, 0, 1, 1]$ | 101,422 | 0.00021 | $[1, 1, 1, 1, 1, 0, 1, 1]$ | 458,876 | 0.00093 |
| $[0, 1, 1, 1, 1, 1, 0, 0]$ | 258,769 | 0.00053 | $[1, 1, 1, 1, 1, 1, 0, 0]$ | 228,059 | 0.00046 |
| $[0, 1, 1, 1, 1, 1, 0, 1]$ | 1,586,548 | 0.00323 | $[1, 1, 1, 1, 1, 1, 0, 1]$ | 1,057,587 | 0.00215 |
| $[0, 1, 1, 1, 1, 1, 1, 0]$ | 252,294 | 0.00051 | $[1, 1, 1, 1, 1, 1, 1, 0]$ | 1,065,182 | 0.00217 |
| $[0, 1, 1, 1, 1, 1, 1, 1]$ | 2,453,351 | 0.00499 | $[1, 1, 1, 1, 1, 1, 1, 1]$ | 8,398,365 | 0.01709 |
| Spike Entropy | | | 4.9319 | | |
| Firing Rate | | | 0.2464 | | |

Table 19: Distribution of the spike patterns in the encoding layer of Spikformer with STF on CIFAR-10 at $T = 8$.

# References

Deng, J.; Dong, W.; Socher, R.; Li, L.-J.; Li, K.; and Fei-Fei, L. 2009. Imagenet: A large-scale hierarchical image database. In *2009 IEEE conference on computer vision and pattern recognition*, 248–255. Ieee.

Deng, S.; Li, Y.; Zhang, S.; and Gu, S. 2022. Temporal efficient training of spiking neural network via gradient reweighting. *arXiv preprint arXiv:2202.11946*.

Goodfellow, I. J.; Shlens, J.; and Szegedy, C. 2014. Explaining and harnessing adversarial examples. *arXiv preprint arXiv:1412.6572*.

He, K.; Chen, X.; Xie, S.; Li, Y.; Dollár, P.; and Girshick, R. 2022. Masked autoencoders are scalable vision learners. In *Proceedings of the IEEE/CVF conference on computer vision and pattern recognition*, 16000–16009.

Horowitz, M. 2014. 1.1 computing's energy problem (and what we can do about it). In *2014 IEEE international solid-state circuits conference digest of technical papers (ISSCC)*, 10–14. IEEE.

Hu, Y.; Tang, H.; and Pan, G. 2021. Spiking deep residual networks. *IEEE Transactions on Neural Networks and Learning Systems*, 34(8): 5200–5205.

Krizhevsky, A.; et al. 2009. Learning multiple layers of features from tiny images.

Li, H.; Liu, H.; Ji, X.; Li, G.; and Shi, L. 2017. Cifar10-dvs: an event-stream dataset for object classification. *Frontiers in neuroscience*, 11: 244131.

Luczak, A. 2024. Entropy of neuronal spike patterns. *Entropy*, 26(11): 967.

Maass, W. 1997. Networks of spiking neurons: the third generation of neural network models. *Neural networks*, 10(9): 1659–1671.

Madry, A.; Makelov, A.; Schmidt, L.; Tsipras, D.; and Vladu, A. 2017. Towards deep learning models resistant to adversarial attacks. *arXiv preprint arXiv:1706.06083*.

Qiu, X.; Zhu, R.-J.; Chou, Y.; Wang, Z.; Deng, L.-j.; and Li, G. 2024. Gated attention coding for training high-performance and efficient spiking neural networks. In *Proceedings of the AAAI Conference on Artificial Intelligence*, volume 38, 601–610.

Yao, M.; Hu, J.; Zhou, Z.; Yuan, L.; Tian, Y.; Xu, B.; and Li, G. 2023. Spike-driven transformer. *Advances in neural information processing systems*, 36: 64043–64058.

Zheng, Z.; Huang, Y.; Yu, Y.; Zhu, Z.; Tang, J.; Yu, Z.; and Jin, Y. 2025. SpiLiFormer: Enhancing Spiking Transformers with Lateral Inhibition. In *Proceedings of the IEEE/CVF International Conference on Computer Vision*.

Zhou, C.; Zhang, H.; Zhou, Z.; Yu, L.; Huang, L.; Fan, X.; Yuan, L.; Ma, Z.; Zhou, H.; and Tian, Y. 2024. QK-Former: Hierarchical Spiking Transformer using QK Attention. *Advances in Neural Information Processing Systems*, 37: 13074–13098.

Zhou, Z.; Zhu, Y.; He, C.; Wang, Y.; Shuicheng, Y.; Tian, Y.; and Yuan, L. 2023. Spikformer: When spiking neural network meets transformer. In *The Eleventh International Conference on Learning Representations*.
